# Supplementary material for: Learning Calibrated Uncertainties for Domain Shift: A Distributionally Robust Learning Approach
Source: arXiv:2010.05784 source file (2024-02-06)
Supplement: Supplementary file 1 [file appendix.tex]

\section{Proof of Lemma \ref{lemma:maxent} and Theorem \ref{thm:para}}
\label{appendix_proof1}
Lemma \ref{lemma:maxent} reduces the original minimax problem into a constrained maximum entropy problem.

\begin{proof} 
We want to solve the following minimax problem:
\begin{align}
\min_{\bm{F}} \; &
\max_{\bm{G} \in \Sigma} \; \mathbb{E}_{\bm{x}\sim\Pt(X)}[-\bm{g}(\bm{x})\cdot\log \bm{f}(\bm{x})] \notag \\
&- r  \mathbb{E}_{\bm{x}\sim \Pt(X)} \left[\bm{y}\odot \bm{g}(\bm{x})\cdot \log \bm{f}(\bm{x})\right]
\end{align}
We first observe that the loss function is convex-concave in terms of $\bm{g}$ and $\bm{f}$. Then we can switch the order of the min player and the max play:
\begin{align}
\max_{\bm{G} \in \Sigma} \; &
\min_{\bm{F}} \;
\mathbb{E}_{\bm{x}\sim\Pt(X)}[-\bm{g}(\bm{x})\cdot\log \bm{f}(\bm{x})] \notag \\
&- r  \mathbb{E}_{\bm{x}\sim \Pt(X)} \left[\bm{y}\odot \bm{g}(\bm{x})\cdot \log \bm{f}(\bm{x})\right]
\end{align}
We then first solve the inner problem and observe that the optimal solution for the inner min problem is $\bm{f} = \bm{g}$. Then we use $\bm{f}$ to replace $\bm{g}$ in the outer max problem and have the following:
\begin{align}
\max_{\bm{F} \in \Sigma} \; &
\mathbb{E}_{\bm{x}\sim\Pt(X)}[-\bm{f}(\bm{x})\cdot\log \bm{f}(\bm{x})] \notag \\
&- r  \mathbb{E}_{\bm{x}\sim \Pt(X)} \left[\bm{y}\odot \bm{f}(\bm{x})\cdot \log \bm{f}(\bm{x})\right]
\end{align}
\end{proof}
We then prove Theorem \ref{thm:para}:
\begin{proof} 
To solve the constrained maximum entropy problem, we first write out the constraints $\bm{f}$ needs to satisfy. $\bm{f}$ needs to reside in the conditional probability simplex and also must satisfy the constraints that $\forall y \in \mathcal{Y}$:
\begin{align}
{\textstyle\sum}_{i} f_y\bm{\phi}(\bm{x}_i)=
{\textstyle\sum}_{i}\mathbb{I}[y_i=y]\bm{\phi}(\bm{x}_i),
\end{align}
where $\bm{x} \sim P_s(\bm{x})$. So before approximating using the finite samples, the constraint can be written as $\forall y \in \mathcal{Y}$:
\begin{align}
 \sum_{\bm{x} \in \mathcal{X}} P_s(\bm{x})f_y(\bm{x})\bm{\phi}(\bm{x})=\sum_{\bm{x} \in \mathcal{X}} P_s(\bm{x}) \bm{g}^y_s(\bm{x})\bm{\phi}(\bm{x}),
\end{align}
where $\bm{g}^y_s(\bm{x})$ denotes the ground-truth conditional distribution in the source data distribution. By the definition of covariate shift, we have $\bm{g}_s(\bm{x}) = \bm{g}_t(\bm{x})$. The right-hand-side is just a fixed vector given the source training data. Therefore, we just use a $\tilde{\bm{c}}_y$ to represent it for each $y$.
The constrained optimization problem then can be written as:
\begin{align}
& \max_{\bm{F}} 
 -\sum_{\bm{x} \in \mathcal{X}} 
 P_{\text{t}}(\bm{x}) \sum_{y \in \mathcal{Y}} f_y(\bm{x})(1 + r \mathbb{I}(y))\log \bm{f}(\bm{x}) \notag\\
& \text{such that: } 
\forall y \in \mathcal{Y}: \sum_{\bm{x} \in \mathcal{X}} {P_\text{s}}(\bm{x}) [f_y(\bm{x}) \bm{\phi}(\bm{x})] = \tilde{ \bm{c}}\notag\\
&\qquad\qquad \text{$\forall \bm{x} \in \mathcal{X}$: }   \sum_{y \in \mathcal{Y}} f_y(\bm{x})=1\notag\\
&\qquad\qquad \text{$\forall \bm{x} \in \mathcal{X}, y \in \mathcal{Y}$: }  f_y(\bm{x})\ge 0.
\end{align}
Note that the final constraint is superfluous since the domain of the
objective function is the positive real numbers.
The Lagrangian associated with this problem is:
\begin{align}
\mathcal{L}&(\theta,\lambda) = \notag \\
& -\sum_{x \in \mathcal{X}} 
 P_{\text{t}}(x) \sum_{y \in \mathcal{Y}}\hat{P}(y|x) (\textbf{1} + r \mathbf{I}(\arg\max_{y'} \hat{P}(y'|x) = y)) \log \hat{P}(y|x) \notag  \\ 
 &+ \sum_k\theta_k\left[\sum_{x \in \mathcal{X}} 
\sum_{y \in \mathcal{Y}}{P_\text{s}}^k(x) \hat{P}(y|x)f_k(x,y)-\tilde{c}_k'
\right] \notag \\
& + \sum_{x \in \mathcal{X}}\lambda(x)\left[\sum_{y \in \mathcal{Y}}\hat{P}(y|x)-1\right],
\end{align}
where $\theta$ and $\lambda(\bm{x})$ are the Lagrangian multipliers. Taking the derivative w.r.t. a specific $f_y(\bm{x})$,
\begin{align}
\frac{\partial}{\partial 
f_y(\bm{x})} \mathcal{L}(\theta,\lambda) = & -P_{\text{t}}(\bm{x})(1 + r \mathbb{I}(y))\log f_y(\bm{x}) -P_{\text{t}}(\bm{x}) \notag \\ 
&+\bm{\theta}_y \cdot{P_\text{s}}(\bm{x})\bm{\phi}(\bm{x})+\lambda(x),
\end{align}

by solving $\frac{\partial}{\partial 
\bm{f}(\bm{x})} \mathcal{L}(\theta,\lambda) = 0$, we get:
\begin{align}
&(1 + r \mathbb{I}(y))\log f_y(\bm{x})) \notag \\
&=-1+\bm{\theta}_y\cdot\frac{{P_\text{s}}(\bm{x})}{P_{\text{t}}(\bm{x})}\bm{\phi}(\bm{x})+\frac{\lambda(\bm{x})}{P_{\text{t}}(\bm{x})} +\frac{(1 + r \mathbb{I}(y))}{P_{\text{t}}(\bm{x})}.
\end{align}

Therefore, we conclude:
\begin{align}
f_y(\bm{x}) \propto e^{\frac{\bm{\theta}_y \cdot\frac{{P_\text{s}}(\bm{x})}{P_{\text{t}}(\bm{x})} \bm{\phi}(\bm{x}) + r \mathbb{I}(y)}{1 + r \mathbb{I}(y)}}.
\end{align}
% with normalization term $Z(x)=\sum_{y \in \mathcal{Y}} e^{\sum_k\frac{{P_\text{s}}^k(x)}{P_{\text{t}}(x)} \theta_k \bm{\phi}(\bm{x})}, \bm{f}(\bm{x})=
% \frac{e^{\sum_k\frac{{P_\text{s}}^k(x)}{P_{\text{t}}(x)} \theta_k \bm{\phi}(\bm{x})}}{Z(x)} $. \\
The derivation of gradient then resembles the derivation in Theorem 1 in \footnote{Anqi Liu and Brian Ziebart. Robust classification under sample selection bias. In Advances in neural information processing systems, pages 37–45, 2014.}.
\end{proof}
%\cite{liu2014robust}.
\begin{figure*}[tb!]
        \centering
        \setlength{\tabcolsep}{-4pt}
        \begin{tabular}{l}
\quad \quad \includegraphics[height=4.2cm]{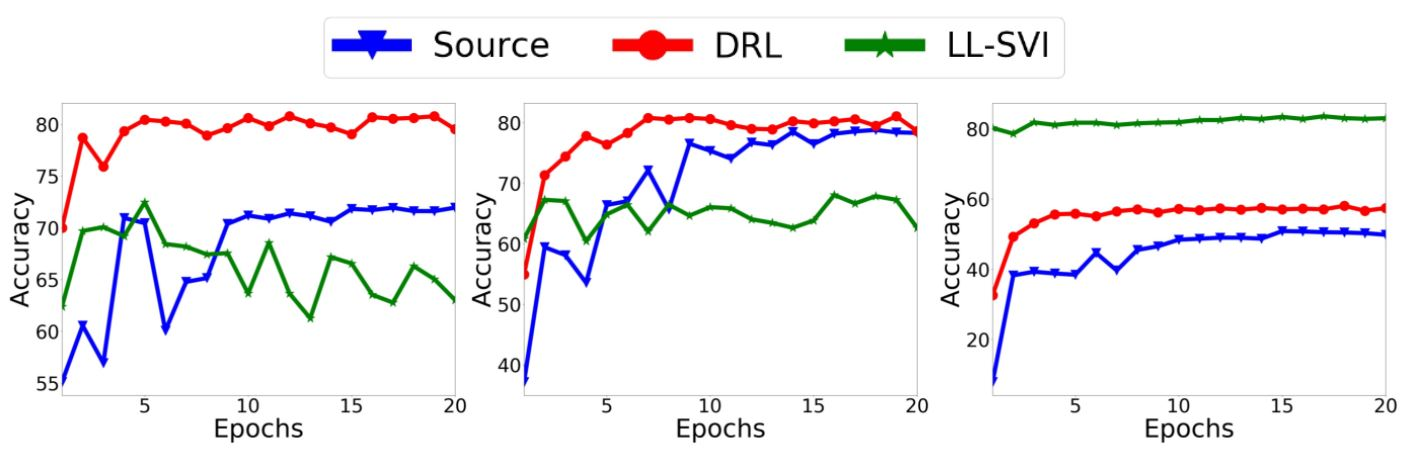}\\
\ \ \quad \quad \quad \quad \quad \quad \quad A$\rightarrow$W  \quad \quad \quad \quad \quad \quad \quad \quad \quad A$\rightarrow$D \ \ \quad \quad \quad \quad \quad \quad \quad \quad \quad W$\rightarrow$A \\
\quad \quad \includegraphics[height=3.3cm]{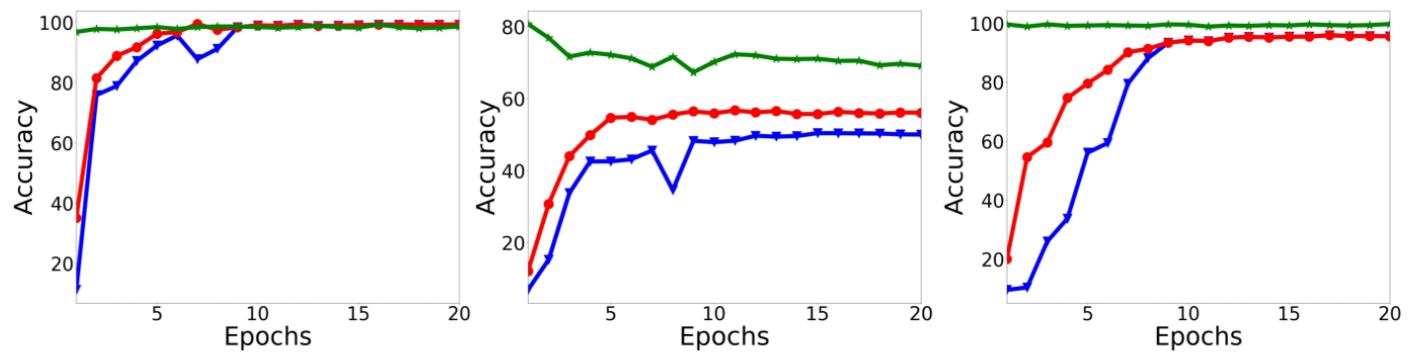}\\
\ \ \quad \quad \quad \quad \quad \quad \quad W$\rightarrow$D  \quad \quad \quad \quad \quad \quad \quad \quad \quad D$\rightarrow$A \ \ \quad \quad \quad \quad \quad \quad \quad \quad \quad D$\rightarrow$W \\
\quad \quad \includegraphics[height=3.3cm]{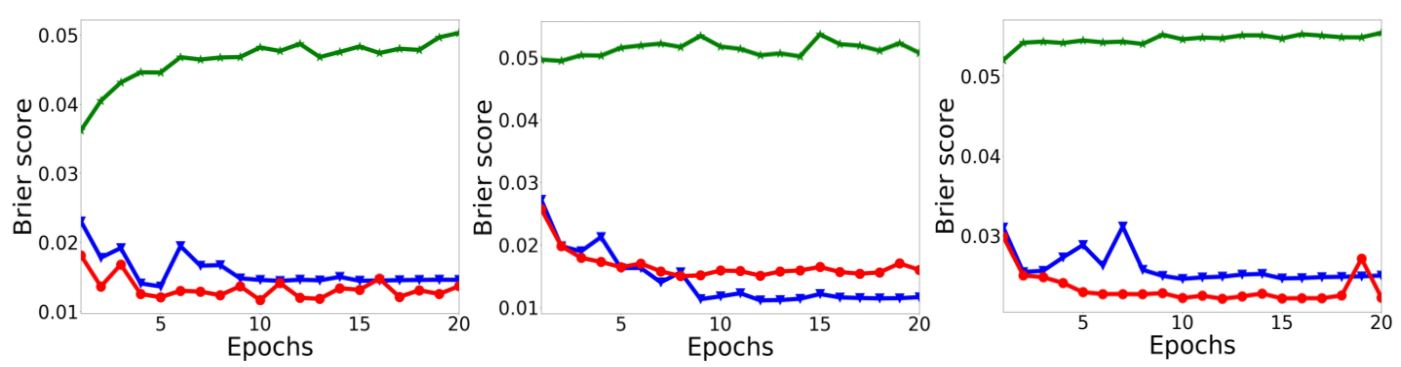}\\
\ \ \quad \quad \quad \quad \quad \quad \quad A$\rightarrow$W  \quad \quad \quad \quad \quad \quad \quad \quad \quad A$\rightarrow$D \ \ \quad \quad \quad \quad \quad \quad \quad \quad \ \ \  W$\rightarrow$A \\
\quad \quad \includegraphics[height=3.3cm]{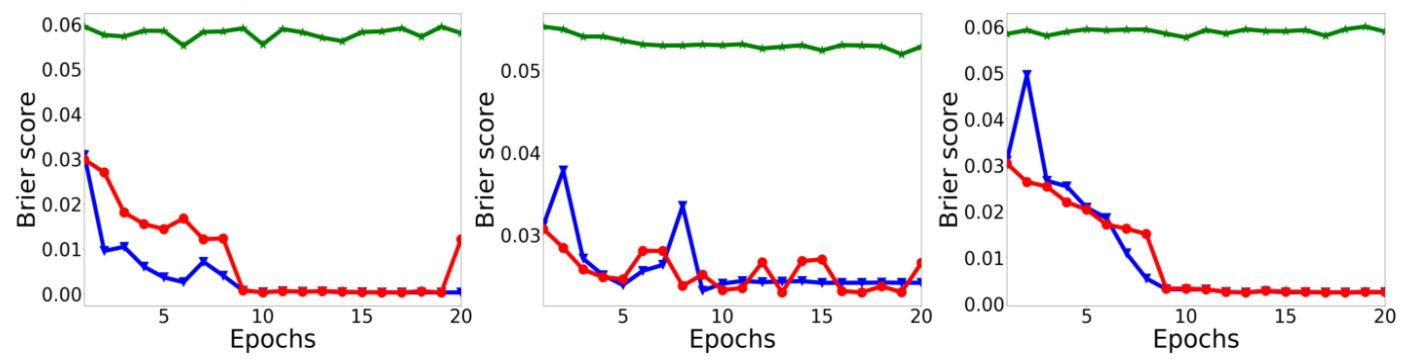}\\
\ \ \quad \quad \quad \quad \quad \quad \quad W$\rightarrow$D  \quad \quad \quad \quad \quad \quad \quad \quad \quad D$\rightarrow$A \ \ \quad \quad \quad \quad \quad \quad \quad \quad \quad D$\rightarrow$W \\
      \end{tabular}
        \vspace{-0.1in}
             \caption{Accuracy and brier score comparison of DRL with source-only and LL-SVI on Office31.}
     \label{fig:brier_all}
    %  \end{tabular}
\end{figure*}

\section{Gradients of the Densities}
\label{appendix_proof2}
As mentioned in the paper, the gradients of the densities come from both of the two loss terms. Let's define the first term $\mathcal{L}_1 \triangleq  \mathbb{E}_{\bm{x}\sim \Pt(X)}\left[-\bm{g}_t(\bm{x})\cdot\log \bm{f}(\bm{x}; \bm{w}_r, \bm{\theta}, \bm{w}_d) \right]$ and the second loss term $\mathcal{L}_2 \triangleq \mathbb{E}_{\bm{x}\sim P_d(X)}\left[-\bm{d}(\bm{x})\cdot\log\bm{\tau}(\bm{x}, \bm{w}_d) \right]$. The gradients of $\mathcal{L}_2$ with respect to $\bm{\tau}$is obvious. Here we only discuss the gradients of $\mathcal{L}_1$ with respect to $\bm{\tau}$. As mentioned in the paper, $\bm{\tau}$ is a two-dimensional vector $(\tau_s, \tau_t)$. We give the gradient for each of them respectively. 

We first show that the first loss term $\mathcal{L}_1$ is equivalent to plugging $\bm{f}$ into the Lagrange $\mathcal{L}(\theta, \lambda)$. Here, for simplicity, we use Eq. \eqref{eq:dratio} as the $\bm{f}(\bm{x})$.
 %\mathbb{E}_{\bm{x}\sim \Pt(X)}\left[-\bm{g}_t(\bm{x})\cdot\log \bm{f}(\bm{x}; \bm{w}_r, \bm{\theta}, \bm{w}_d) \right] + \mathbb{E}_{\bm{x}\sim P_d(X)}\left[-\bm{d}(\bm{x})\cdot\log\bm{\tau}(\bm{x}, \bm{w}_d) \right]
% \begin{equation}
% 	\begin{split}
% 	\frac{\partial \mathcal{L}_1}{\partial } &= \frac{\partial}{\partial R}\left(-\theta \cdot \mathbb{E}_{P_\text{s}(x)P(y|x)}[\Phi(X, Y)] + \mathbb{E}_{P_\text{t}(x)}[\log Z_{\theta}(X)]\right)\\ &=
% 	\mathbb{E}_{P_\text{t}(x)}\left[\mathop{\sum}_{y \in Y} \frac{\exp(R, \theta, \Phi)}{Z_{\theta}(X)} \theta \cdot \Phi(X, Y)\right] = ,
% 	\end{split}
% \end{equation}
\begin{align}
\mathcal{L}(\theta, \lambda)=& -\sum_{\bm{x} \in \mathcal{X}} 
 P_{\text{t}}(\bm{x}) \sum_{y \in \mathcal{Y}}f_y(\bm{x})\cdot
\left(\bm{\theta}_y \cdot \frac{\Ps(\bm{x})}{P_{\text{t}}(\bm{x})} \bm{\phi}(\bm{x})-\log Z_{\bm{\theta}}(\bm{x})\right)\notag\\
&+ \left[ \sum_{y \in \mathcal{Y}} \bm{\theta}_y \cdot \sum_{\bm{x} \in \mathcal{X}} 
\Ps(\bm{x})f_y(\bm{x})\bm{\phi}(\bm{x})-\tilde{\bm{c}}_y\right]\notag\\
=&\sum_{\bm{x} \in \mathcal{X}}P_{\text{t}}(\bm{x})\log Z_{\bm{\theta}}(\bm{x})- \sum_{y \in \mathcal{Y}} \bm{\theta}_y \cdot \tilde{{\bf c}}_y.
\end{align}
On the other hand, 
\begin{align}
    \mathcal{L}_1 & = \mathbb{E}_{\bm{x}\sim \Pt(X)}\left[-\bm{g}_t(\bm{x})\cdot\log \bm{f}(\bm{x}) \right] \notag \\
    & = \sum_{\bm{x} \in \mathcal{X}}P_{\text{t}}(\bm{x})\log Z_{\bm{\theta}}(\bm{x})- \sum_{\bm{x} \in \mathcal{X}} P_{\text{t}}(\bm{x}) \sum_{y\in \mathcal{Y}}g^y_t(\bm{x})\bm{\theta}_y \cdot \frac{\Ps(\bm{x})}{P_{\text{t}}(\bm{x})} \bm{\phi}(\bm{x}) \notag \\
    & = \sum_{\bm{x} \in \mathcal{X}}P_{\text{t}}(\bm{x})\log Z_{\bm{\theta}}(\bm{x})-\sum_{y\in \mathcal{Y}} \bm{\theta}_y \cdot \tilde{{\bf c}}_y \notag \\
    & = \mathcal{L}(\theta, \lambda)
\end{align}
Then, we take the derivative of a specific $\bm{x}$'s densities, $\tau_s(\bm{x})$ and $\tau_t(\bm{x})$.
=
\begin{align}
\frac{\partial \mathcal{L}_1}{\partial \tau_s} &= \frac{\partial}{\partial \tau_s}\left(\sum_{\bm{x} \in \mathcal{X}}P_{\text{t}}(\bm{x})\log Z_{\bm{\theta}}(\bm{x})-\sum_{y \in \mathcal{Y}} \bm{\theta}_y \cdot \tilde{{\bf c}}_y\right) \notag \\
& = \frac{1}{\tau_t} \sum_{\bm{x} \in \mathcal{X}}P_{\text{t}}(\bm{x}) \sum_{y \in \mathcal{Y}}  \bm{\theta}_y \cdot \frac{\exp( \bm{\theta}_y\cdot  \frac{\Ps(\bm{x})}{\Pt(\bm{x})} \bm{\phi}(\bm{x}))}{Z_{\bm{\theta}}(\bm{x})}  \bm{\phi}(\bm{x}) \notag \\
&= \frac{1}{\tau_t}\mathbb{E}_{\bm{x}\sim P_t(X)}\left[\sum_{y  \in \mathcal{Y}}\bm{\theta}_y \cdot  f_y(\bm{x}) \bm{\phi}(\bm{x})\right].
\end{align}

In the same spirit, the gradient of $\mathcal{L}_1$ over target densities $\tau_t$ is:

\begin{align}
\frac{\partial \mathcal{L}_1}{\partial \tau_t} &= \frac{\partial}{\partial \tau_t}\left(\sum_{\bm{x} \in \mathcal{X}}P_{\text{t}}(\bm{x})\log Z_{\bm{\theta}}(\bm{x})- \sum_{y \in \mathcal{Y}} \bm{\theta}_y \cdot \tilde{{\bf c}}_y\right) \notag\\
& = \frac{\tau_{s}}{\tau_{t}^2}  \sum_{\bm{x} \in \mathcal{X}}P_{\text{t}}(\bm{x}) \sum_{y \in \mathcal{Y}} \bm{\theta}_y \cdot \frac{\exp( \bm{\theta}_y\cdot \frac{\Ps(\bm{x})}{\Pt(\bm{x})} \bm{\phi}(\bm{x}))}{Z_{\bm{\theta}}(\bm{x})}  \bm{\phi}(\bm{x}) \notag\\
&= \frac{\tau_{s}}{\tau_{t}^2} \mathbb{E}_{\bm{x}\sim P_t(X)}\left[\sum_{y  \in \mathcal{Y}}\bm{\theta}_y \cdot  f_y(\bm{x}) \bm{\phi}(\bm{x})\right].
\end{align}

Here, $f_y$ is the $y$-th dimension of the prediction $\bm{f}$ and $Z_{\bm{\theta}}(\bm{x})$ is the normalization term of $\bm{f}$. Note that, the gradients are not relevant to the target labels, but only target input data. We then use finite samples in the target domain to approximate these gradients.  

\section{Algorithm}
\label{appendx:alg}
In this part, we summarize our parameter learning process, as proposed in Section 2.3. Algorithm \ref{alg:endtoend} shows the details.
\begin{algorithm}[H]
\caption{End-to-end Training for DRL}
\label{alg:endtoend}
\begin{small}
\begin{algorithmic}[1]
\STATE {\bfseries Input}: DNN $\bm{\phi}$ and DNN $\bm{\tau}$, with optimizer SGD$_1$ and SGD$_2$, respectively. Learning rates $\gamma_1$ and $\gamma_2$, epoch number $T$.
\STATE {\bfseries Initialization}: $\bm{\phi}, \bm{\tau} \leftarrow$ random initialization, epoch $\leftarrow 0$
\STATE {\bfseries While} epoch $< T$
\STATE \qquad {\bfseries For} each data mini-batch
\STATE \qquad\qquad Update $\bm{\tau}$ by SGD$_1(\gamma_1)$ using the combined gradients from both loss terms in Eq. \ref{eq:joint_loss};
\STATE \qquad\qquad Compute $\bm{f}$ using $\bm{\theta}$, $\bm{w}_r$, and $\bm{w}_d$;
\STATE \qquad\qquad Update $\bm{\phi}, \bm{\theta}$ by SGD$_2(\gamma_2)$ using derived gradients;
\STATE \qquad epoch $\leftarrow$ epoch $+1$
\STATE {\bfseries Output}: Trained networks $\bm{\phi}$, $\bm{\tau}$.
\end{algorithmic}
\end{small}
\end{algorithm}

\begin{figure*}[tb!]
        \centering
        \setlength{\tabcolsep}{-5pt}
        \begin{tabular}{cccc}
\includegraphics[height=3.1cm, ]{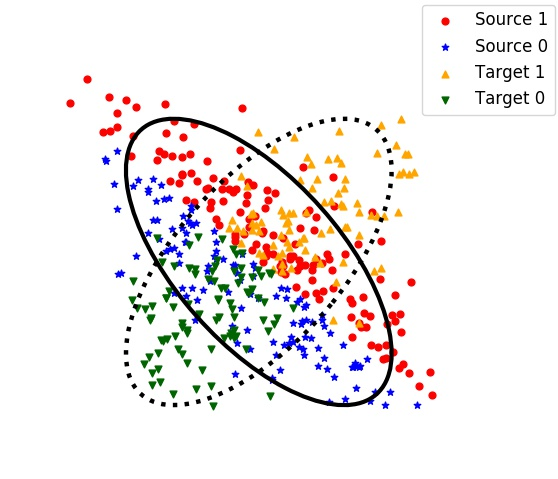}& \quad
\includegraphics[height=3.1cm, ]{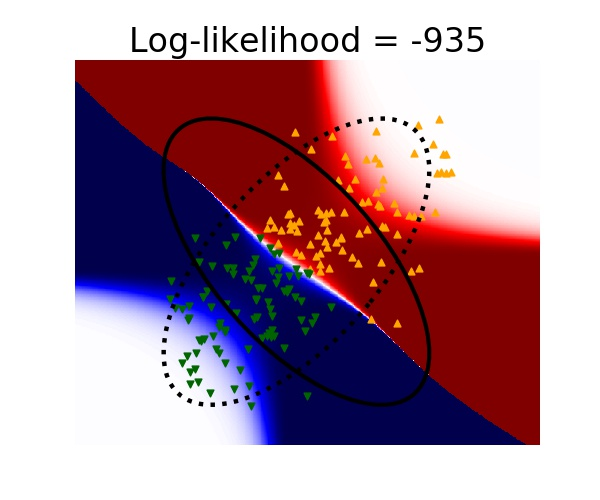}& \quad
\includegraphics[height=3.1cm, ]{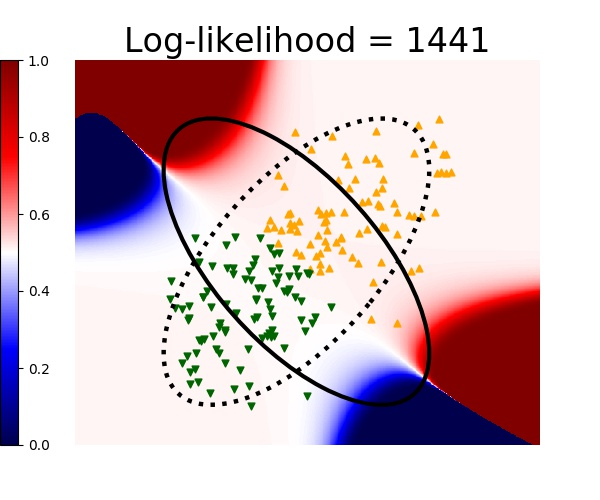}& \quad
\includegraphics[height=3.1cm, ]{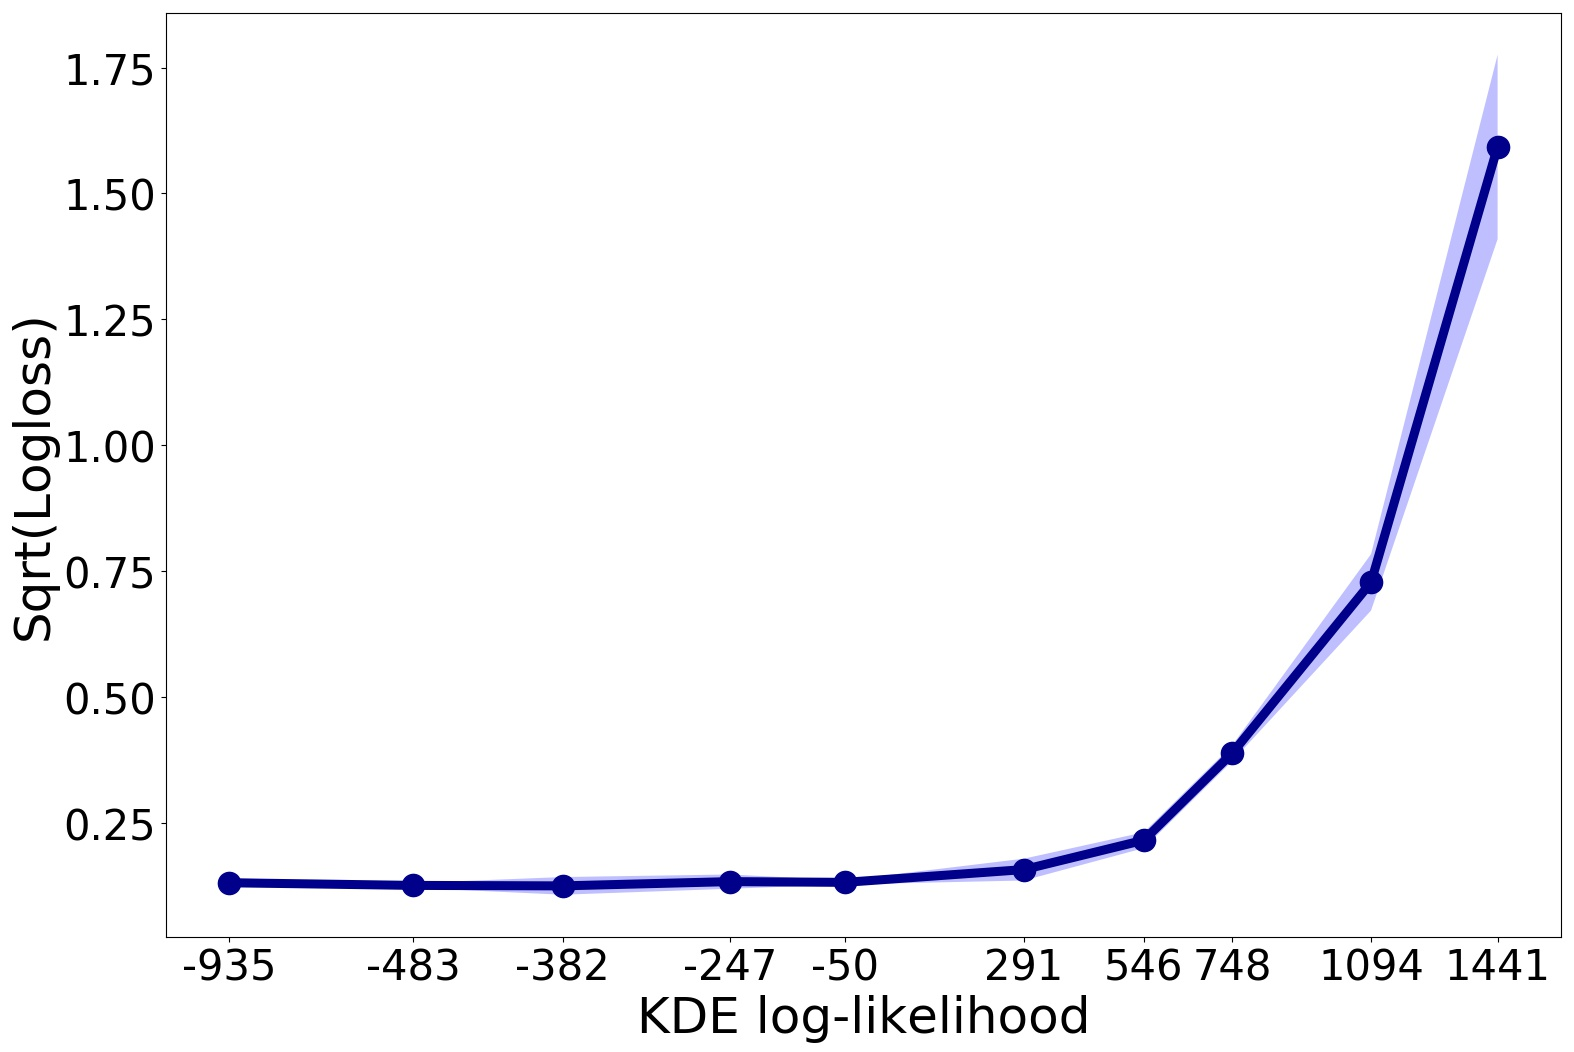}\\
(a)&(b)&(c)&(d)
      \end{tabular}
        \vspace{-0.1in}
             \caption{(a) Source and target data points are drawn from two Gaussian distributions. Solid line: source, dashed line: target. The underlying true decision boundary for the binary classes is the same between the two domains. (b)-(c) Prediction with density ratios from low and high density estimation likelihoods. With more accurate density estimation, the RBA predictor gives overly conservative predictions on the target domain. The colormap is the confidence $P(``1"|x)$. (d) With larger likelihood in density estimation, the target log loss becomes worse.}
     \label{fig:2d}
\end{figure*}

\section{Further Discussion of Related Works}
\subsection{Comparison with pseudo-label generation methods}
Different from ReMixMatch, FixMatch and AdaMatch, our pseudo-labels are assigned directly according to the uncertainties generated by the distributionally robust learning approach. In particular, the three methods generate and modify pseudo-labels in two-stage: estimate the pseudo-label distribution and align it with the ground-truth distribution, or augment data differently and align the predictions. Yet our method directly generates calibrated predictions

\subsection{Comparison with calibration methods}
Our uncertainty is generated implicitly, and is not competitive of methods that directly aim for uncertainty calibration, such as TransCal (X.Wang, M. Long, J. Wang, and M. Jordan. Transferable Calibration with Lower Bias and Variance in Domain Adaptation. In NeurIPS, 2020). We mainly compare with other relative methods that faces the target task of unsupervised domain adaptation (instead of better calibration), and better calibration is an inherent property of our method, as well as an explaination for better performance of our method when using self-training.

\section{Simulation on the plug-in estimator for the density ratios}
\label{app:plugin}
The density ratios are important factors adjusting the representation-level conservativeness for DRL. Like many other machine learning methods using density ratios such as, transfer learning \footnote{Sinno Jialin Pan and Qiang Yang. A survey on transfer learning. IEEE Transactions on knowledge and data engineering, 22(10):1345–1359, 2009.} %\citep{pan2009survey}
, and off-policy evaluation \footnote{Miroslav Dudík, John Langford, and Lihong Li. Doubly robust policy evaluation and learning. arXiv preprint arXiv:1103.4601, 2011.} 
%\citep{dudik2011doubly}
, we can use a plug-in estimator for the density ratio $\Ps(\bm{x}) /\Pt(\bm{x}) $. However, density ratio estimation \footnote{Masashi Sugiyama, Taiji Suzuki, and Takafumi Kanamori. Density ratio estimation in machine learning. Cambridge University Press, 2012.}
%\citep{sugiyama2012density}
, especially in the high-dimensional data, is rather difficult. Here, we ask the question: \textbf{whether a more accurate density ratio estimate leads to a greater predictive performance in the downstream tasks?}

We show a two-dimensional binary classification example in Figure \ref{fig:2d} to demonstrate relation between the performance of the density (ratio) estimation and the performance of the ultimate target learning tasks. Kernel density estimation (KDE) is conducted to evaluate the average log-likelihood of the source and target data on the source and target distributions. We take the ratio of the density from KDE to replace the output of the density ratio estimator. We can see that the case with higher log-likelihood actually fails to give informative predictions on the target classification task. The main reason is that the density (ratio) estimation task, as an independent learning task, does not share information with the downstream prediction tasks that use the ratios. Therefore, if the density ratio estimation over-optimize for its own objective, it may even hurts the performance for the downstream tasks.

\section{Additional Results}
\label{appendix_results}
In this section, we provide results for DRL, DRST and DRSSL in addition to Sec. \ref{sec:exp}. 

\subsection{Additional DRL Results (for Section 3.1)}
\subsubsection{Accuracy Comparison of DRL on Office31.} Note that DRL not only achieves better uncertainties than the baselines, but also does not hurt the prediction accuracy too much and may even achieve better accuracy. We show the DRL results on all of the tasks of Office31 in Figure~\ref{fig:brier_all} by comparing accuracy with Source model and a Bayesian method: LL-SVI \footnote{Riquelme, C., Tucker, G., and Snoek, J. Deep Bayesian Bandits Showdown: An Empirical Comparison of Bayesian Deep Networks for Thompson Sampling. In ICLR, 2018.}.

\subsubsection{Additional Brier Score Results on Office31.}  Figure~\ref{fig:brier_all} (Bottom) also demonstrates that our method generate more calibrated uncertainty estimates than Source and LL-SVI.

\subsubsection{Additional Reliability Plots on Office31.} Figure~\ref{fig:reliability_office} shows all the reliability plots in all tasks in Office31 (blue line for source-only, green line for TS and orange line for DRL).

\begin{figure*}[tb!]
        \centering
        \setlength{\tabcolsep}{-4pt}
        \begin{tabular}{ccc}
\includegraphics[height=2.7cm]{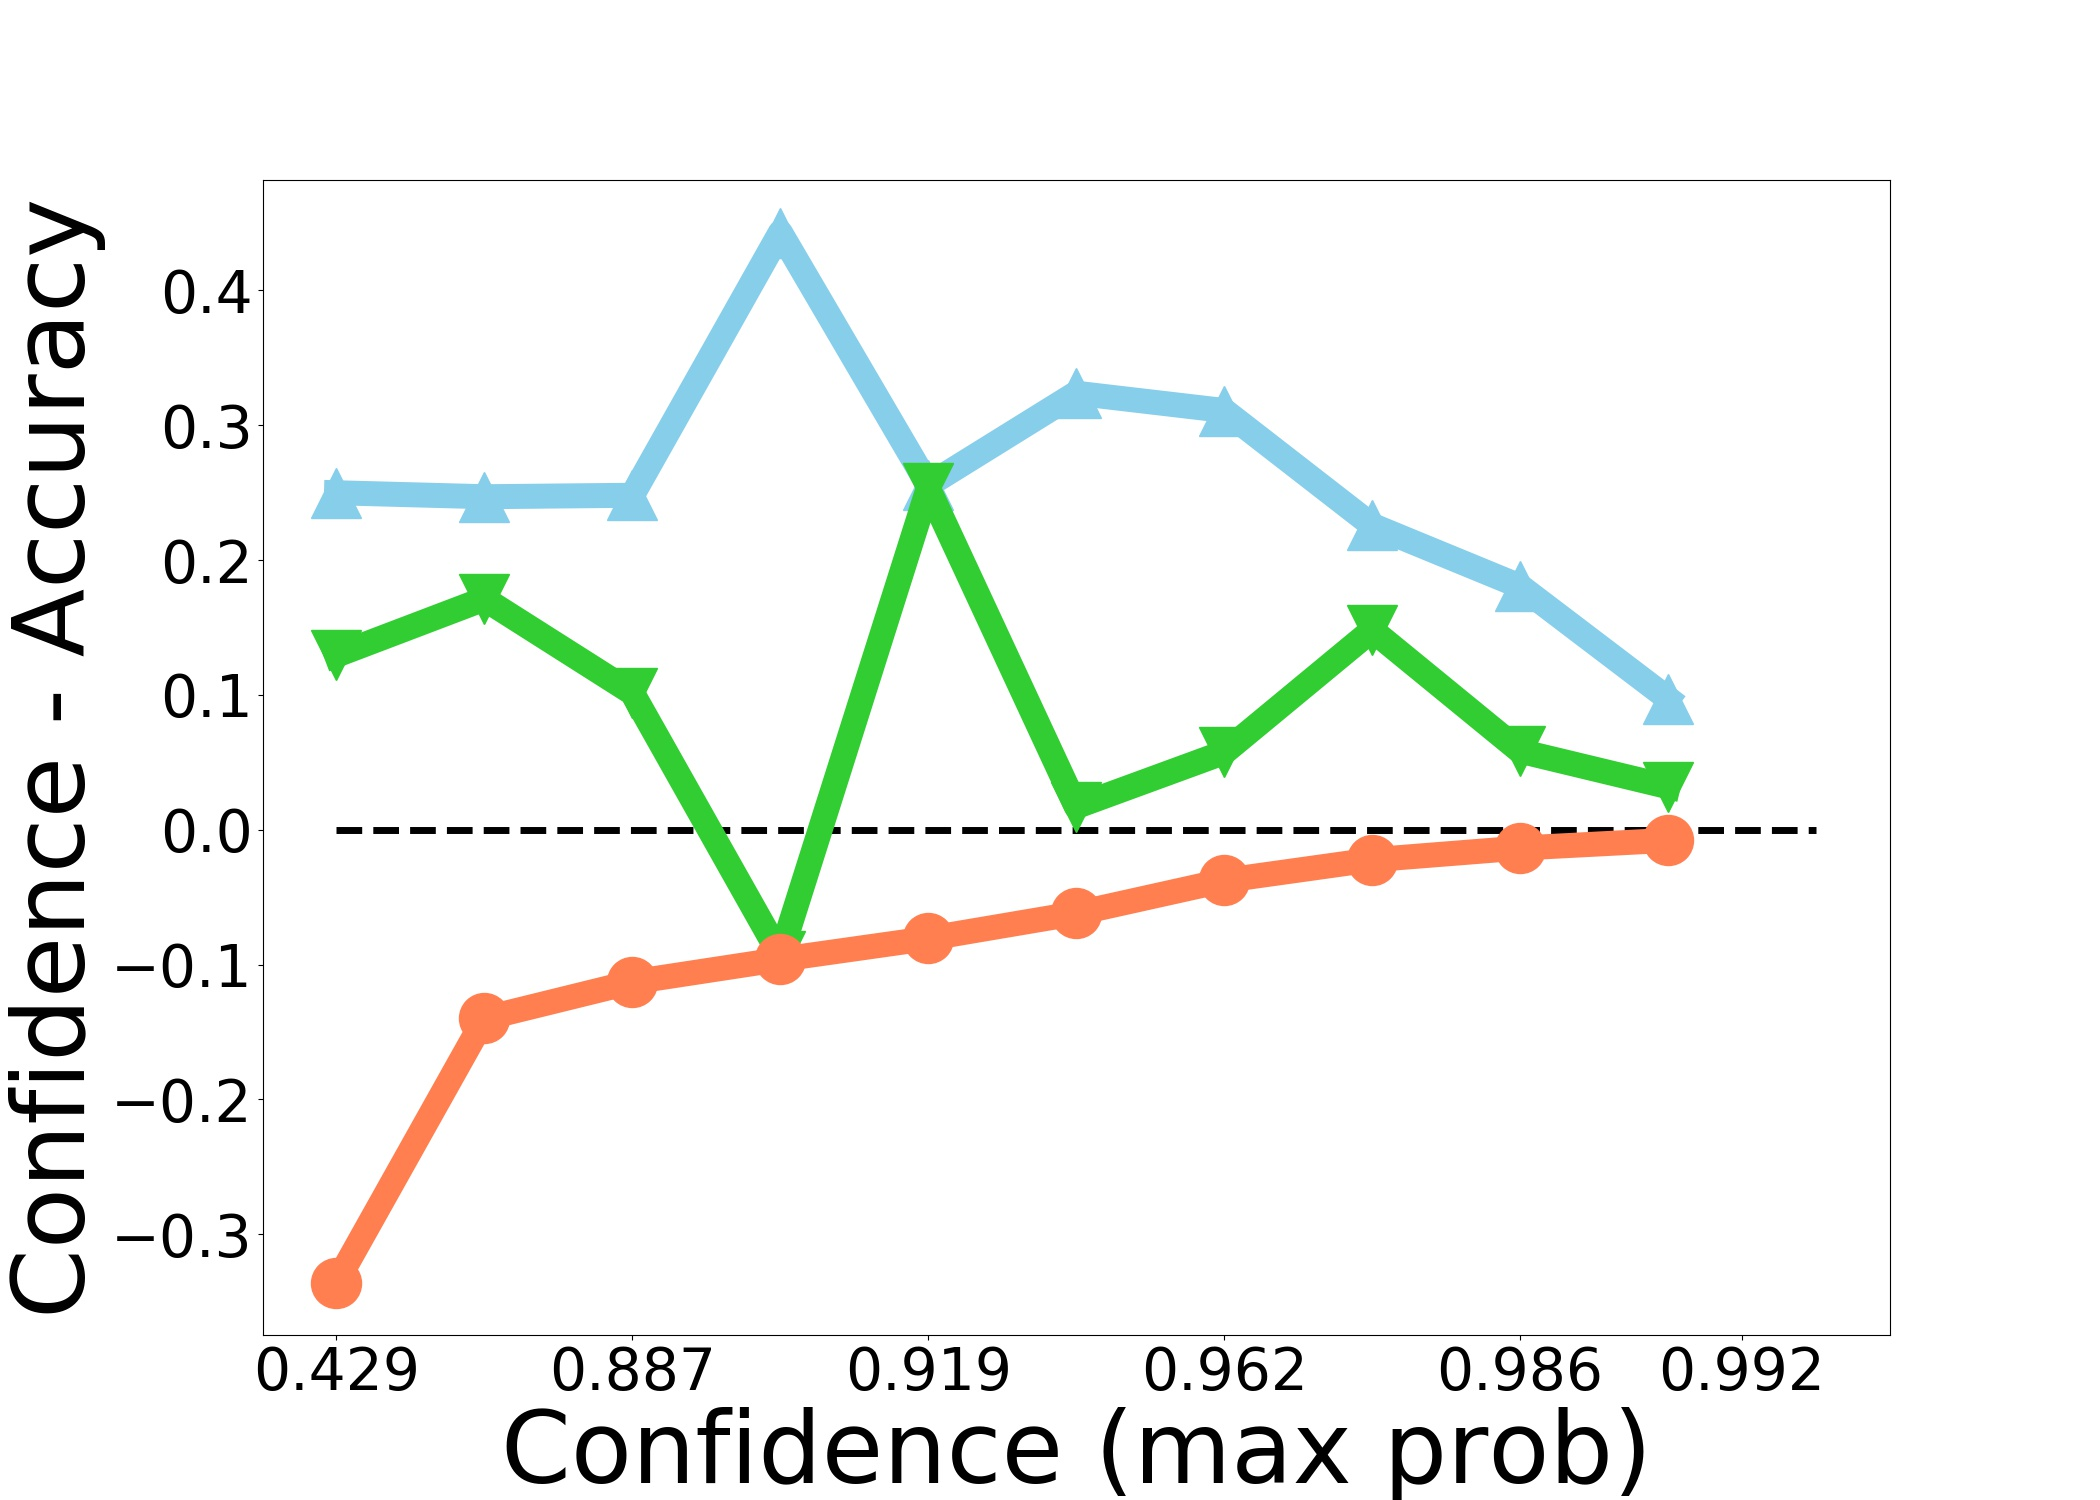}& \quad \quad \quad \quad
\includegraphics[height=2.7cm]{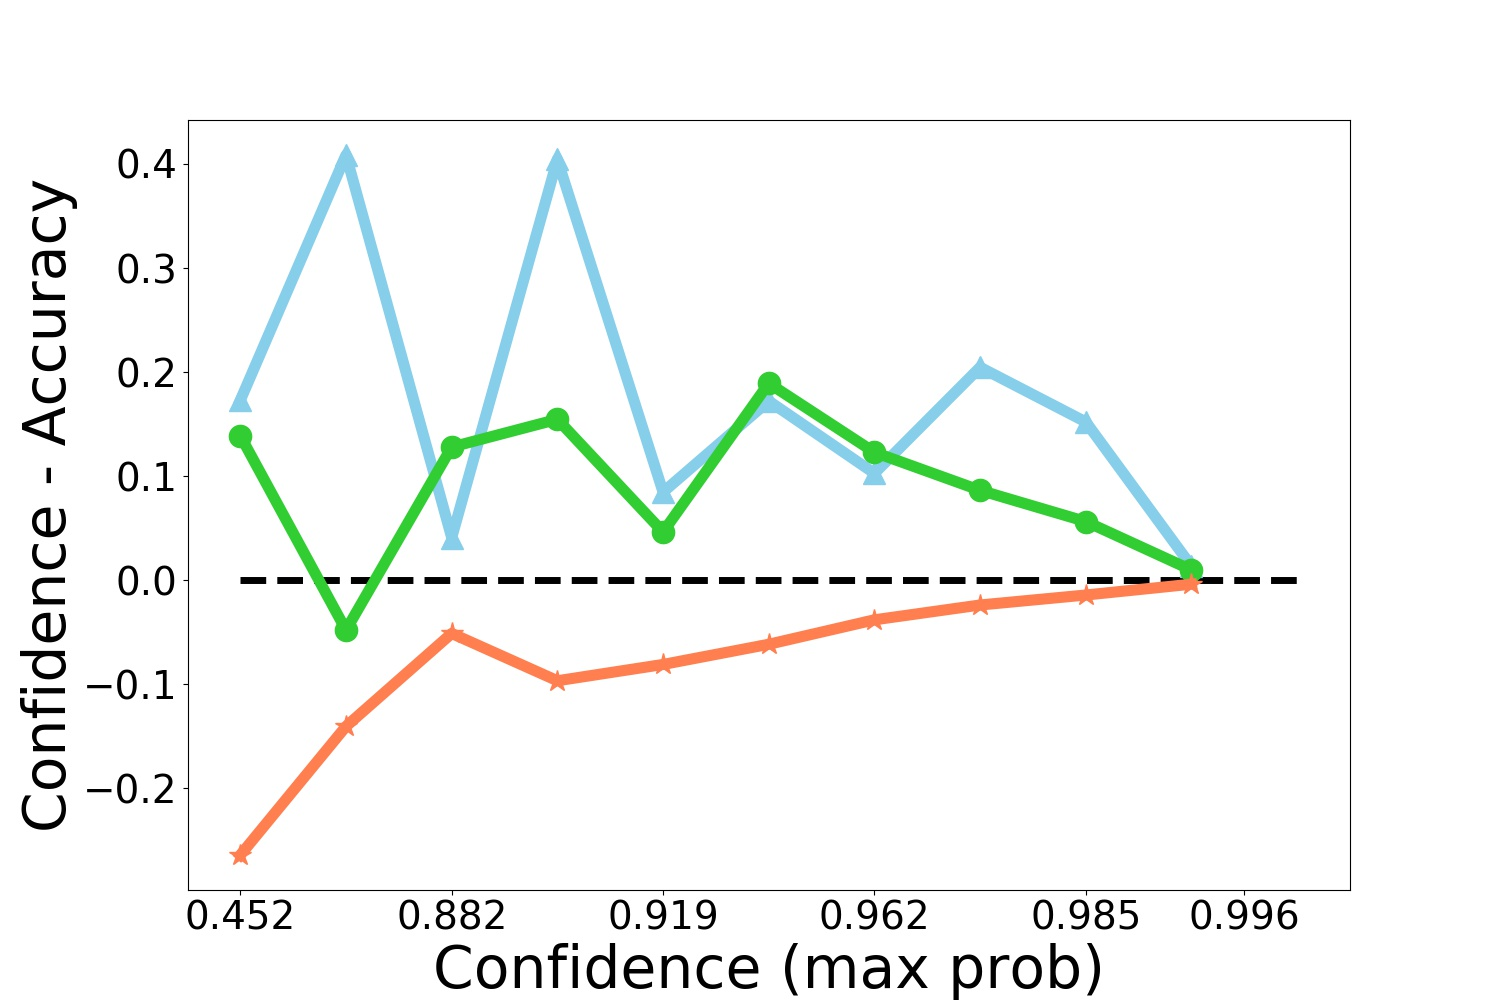}& \quad \quad \quad \quad 
\includegraphics[height=2.7cm]{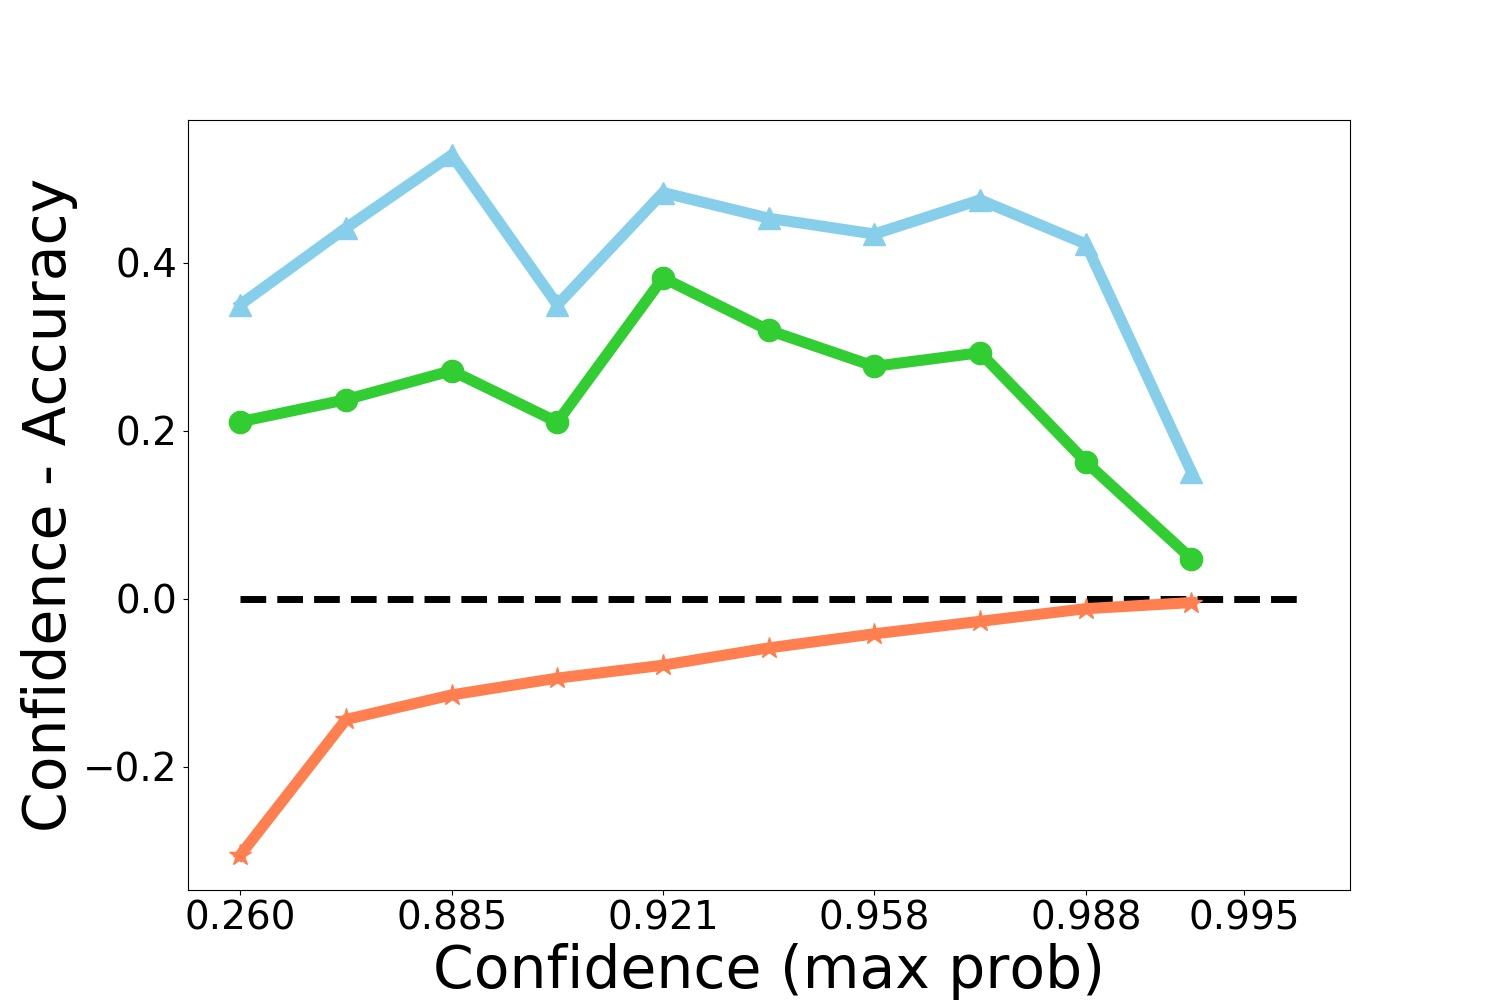} \\ 
\includegraphics[height=2.7cm]{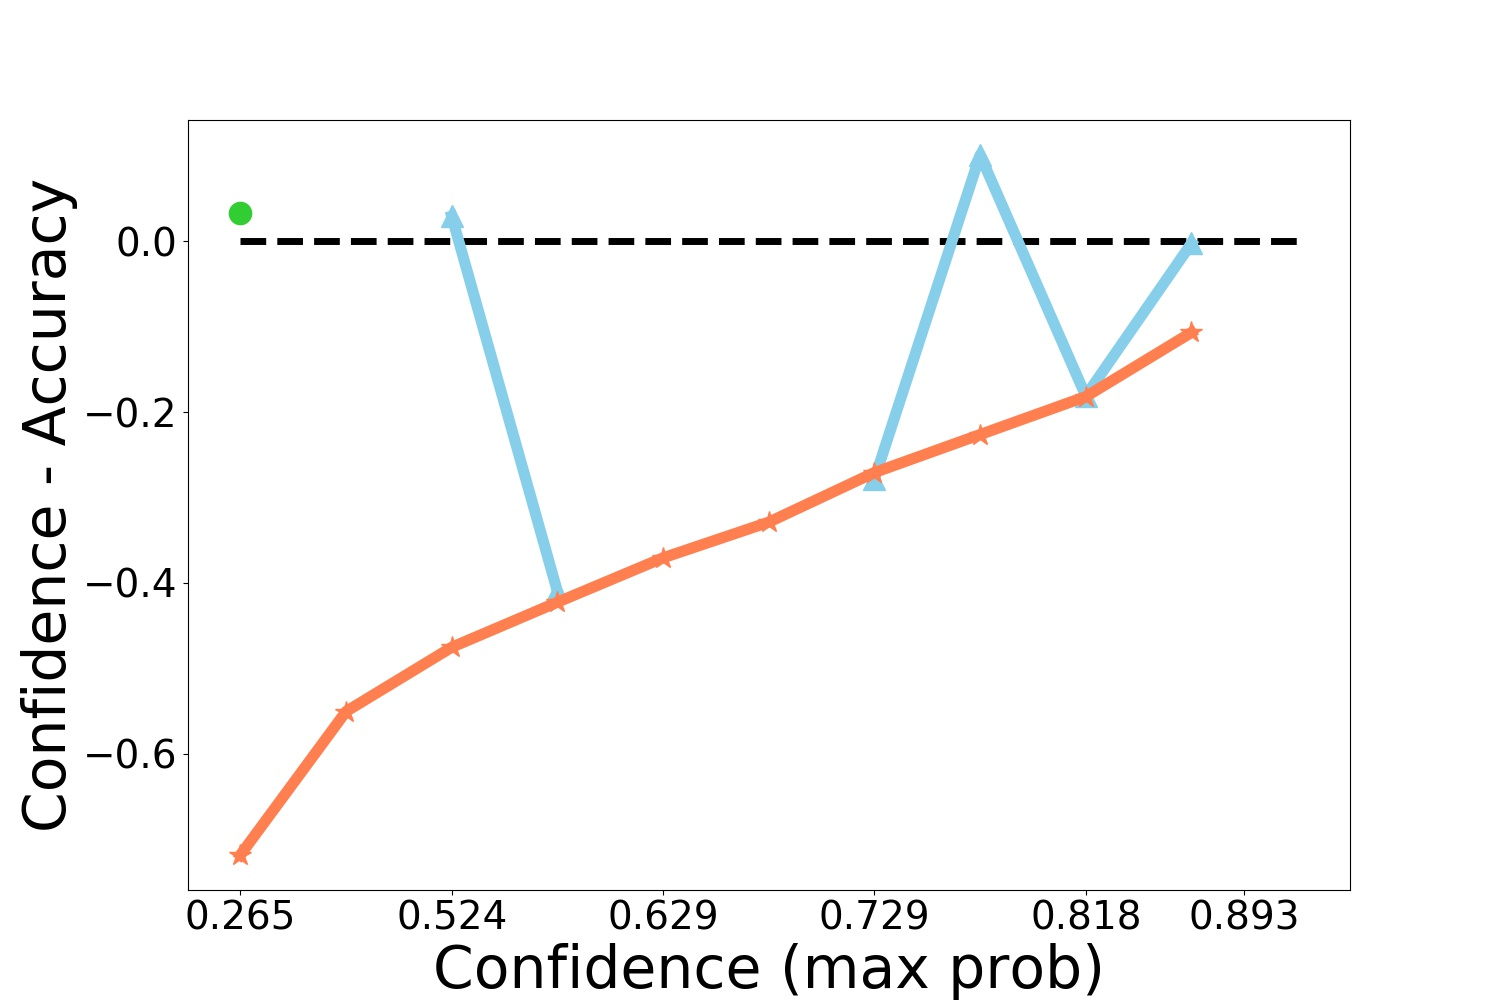}& \quad \quad \quad \quad 
\includegraphics[height=2.7cm]{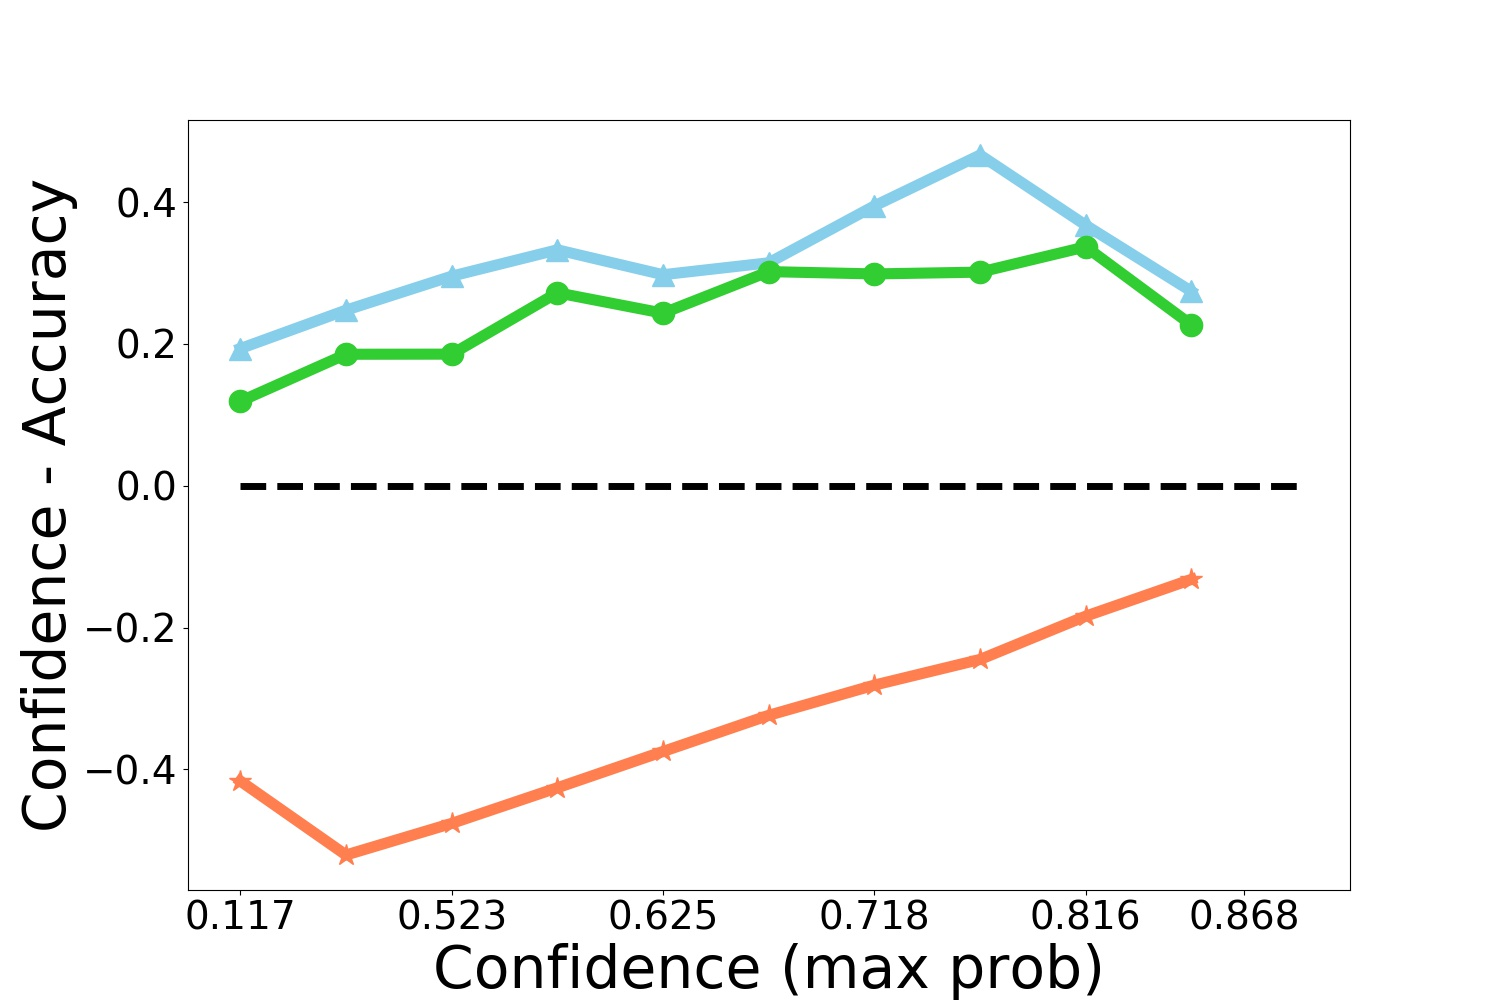}& \quad \quad \quad \quad 
\includegraphics[height=2.7cm]{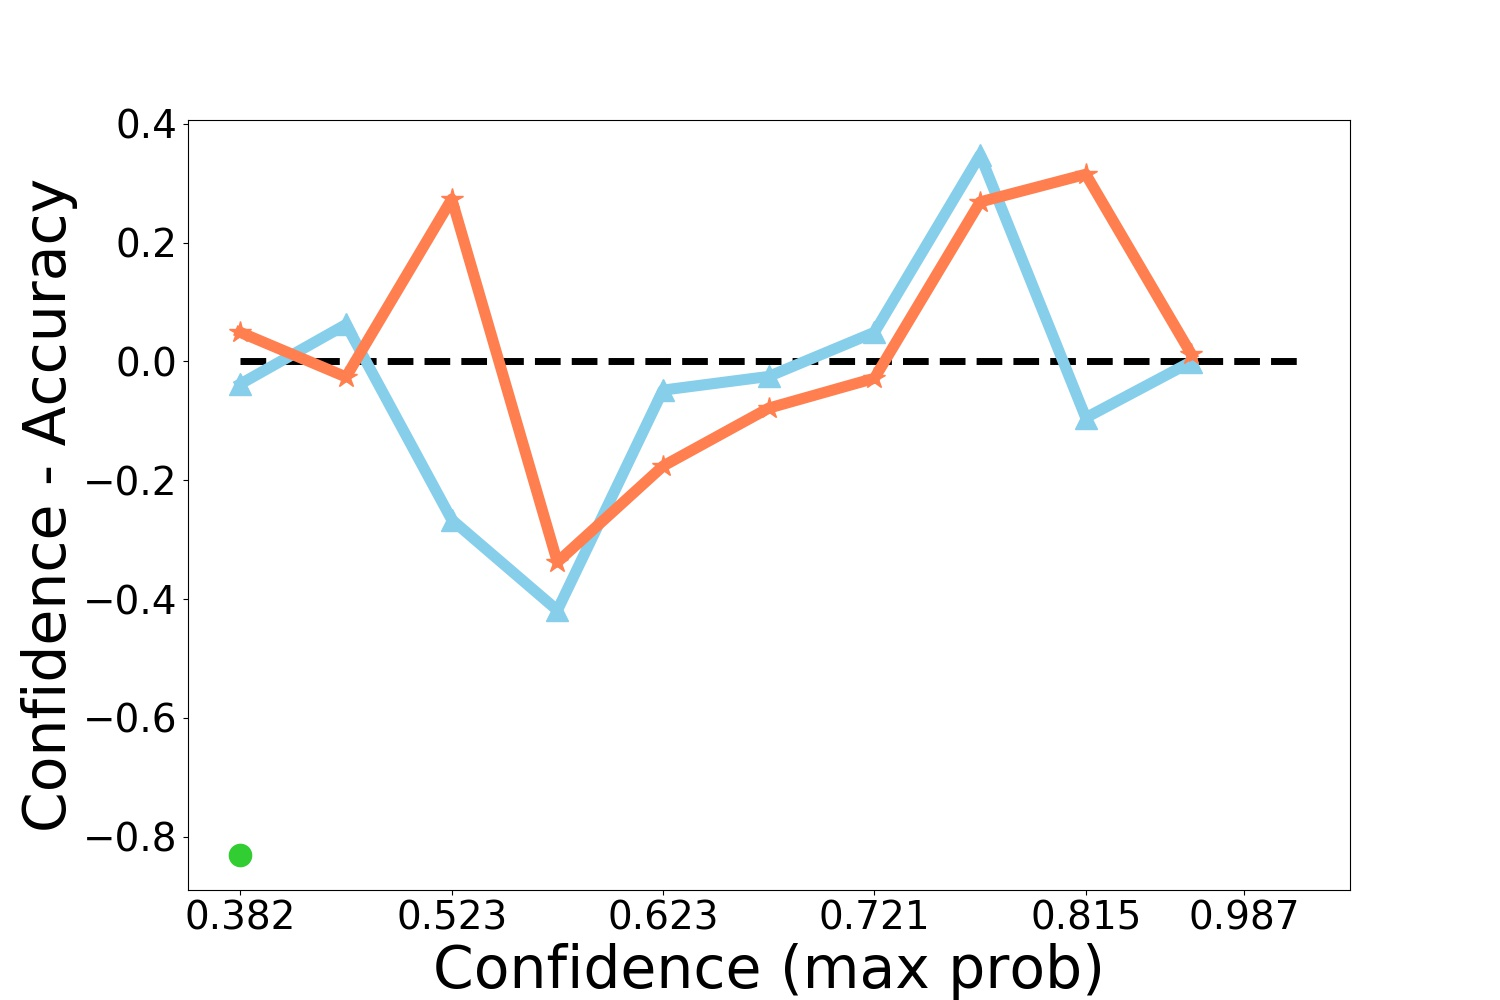} \\
\quad (a)& \ \ \quad \quad \quad \quad \quad (b)& \ \ \quad \quad \quad \quad \quad (c) \\
      \end{tabular}
        \vspace{-0.1in}
             \caption{Office31 results on reliability plots, which is a complement for Figure 4 in main text. DRL is compared with source-only and temperature scaling. Note that there are some missing points for source-only and TS in some plots. This is due to the fact that the corresponding models do not have data prediction results with confidence in those ranges.}
     \label{fig:reliability_office}
    %  \end{tabular}
\end{figure*}

\begin{figure*}[htb]
        \centering
        \setlength{\tabcolsep}{-4pt}
        \begin{tabular}{l}
\includegraphics[height=3.5cm]{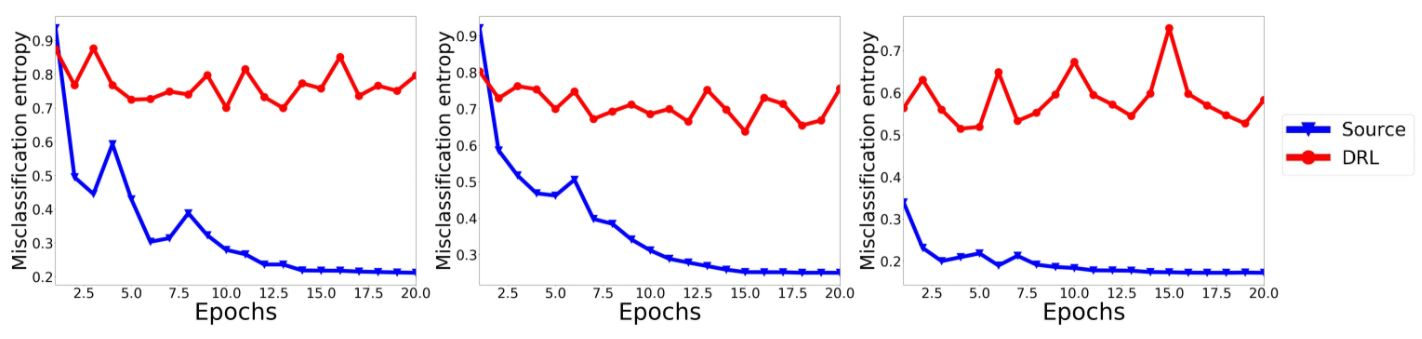}\\
\quad \quad \quad \ \  Office31 (A$\rightarrow$W) \quad \quad \quad \quad \ \ Office-Home (P$\rightarrow$A) \quad \quad \quad \quad \quad \quad \ \  VisDA
      \end{tabular}
        \vspace{-0.1in}
             \caption{Comparison of DRL and source-only of misclassification entropy on different datasets.}
     \label{fig:misent}
    %  \end{tabular}
\end{figure*}

\subsubsection{Misclassification Entropy Comparison on Office31.} Figure~\ref{fig:misent} shows the misclassification entropy comparison between source model and the DRL model. Misclassification entropy is calculated as $S_{i} = \frac{1}{n}\mathop{\sum}_{i=1}^{n} \mathop{\sum}_{j=1}^{m} p_{ij} \log p_{ij}$ , where $n$ is the number of samples and $m$ is the number of categories in the dataset, and $p_{ij}$ indicates the prediction probability of the $i$th sample on the $j$th category. The larger misclassification entropy is, the more uncertain the model prediction result is on the wrong predictions. This means the model would fail more gently. 

\subsubsection{ECE Results on VisDA.} 
%Table \ref{tab:ece_office} demonstrates the expected calibration error of Source-Only, LL-SVI , TS and our method on different tasks in the Office31 datasets. LL-SVI is an approximate Bayesian inference method for the parameters of the last layer only. DRL achieves much better ECE than all the baselines. 
Table \ref{tab:ece_visda} shows the ECE scores and corresponding accuracies on VisDA2017 for Source-Only, TS and DRL. TS here uses the target set for calibration thus is the oracle for the metrics. We do not adopt self-training here. We can see that in terms of calibration, DRL is near the oracle performance. 

\iffalse
\begin{table}[b]
\centering
\caption{ECE score comparison on Office31}
\begin{tabular}{ccccccc}
\toprule
Tasks & A$\rightarrow$W & A$\rightarrow$D & W$\rightarrow$A & W$\rightarrow$D & D$\rightarrow$A & D$\rightarrow$W \\ 
\midrule
Source-Only & 0.175 & 0.105 & 0.309 & 0.006 & 0.280 & 0.029 \\ 
LL-SVI      & 0.201 & 0.193 & 0.082 & 0.010 & 0.153 & 0.006 \\ 
TS          & 0.088 & 0.086 & 0.192 & 0.033 & 0.218 & 0.838 \\ 
DRL         & 0.300 & 0.216 & 0.299 & 0.547 & 0.417 & 0.024 \\ \bottomrule
\end{tabular}
\label{tab:ece_office}
\end{table}
\fi

\begin{table}[h]
\centering
\begin{tabular}{cccc}
\toprule
Methods & Source-Only & TS & DRL  \\
\midrule
ECE    & 9.58  & 2.15 & 2.14\\
Accuracy (\%) & 55.04 & 62.84  & 77.07\\
\bottomrule
\end{tabular}
\caption{ECE score comparison on VisDA2017}
\label{tab:ece_visda}
\end{table}

\subsubsection{Full density Ratio Results for Different HSF Bins on ImageNetV2.} When comparing the density ratios of different HSFs (Figure 5), we treat low HSF as having HSF in range $[0, 0.2]$, and high HSF from $(0.2, 1]$. Results on ResNet50 and DenseNet121 are shown in Table \ref{tab:dr_hsf1}. We also show more detailed comparison between density ratio and HSF. Here we divide the HSF into 5 bins, with ranges of $[0.0,0.2]$, $[0.2, 0.4]$, $[0.4,0.6]$, $[0.6, 0.8]$,$[0.8, 1.0]$. We show the numbers in Table \ref{tab:dr_hsf2}. Note that the numbers might be inconsistent with the binary case, because we calculated the numbers based on different models for variance.
\begin{table}[h]
    \centering
    \begin{tabular}{ccc}
        \toprule
        HSF & ResNet50 & DenseNet121 \\
        \midrule
        Low HSF & 1.797 & 0.657 \\
        High HSF & 1.804 & 0.665 \\ 
        \bottomrule
    \end{tabular}
    \caption{Additional results on density ratio v.s. HSF}
    \label{tab:dr_hsf1}
\end{table}

\begin{table}[h]
    \centering
    \resizebox{0.48\textwidth}{9.5mm}{
    \begin{tabular}{cccccc}
        \toprule
        HSF & [0.0, 0.2] & [0.2, 0.4] & [0.4, 0.6] & [0.6, 0.8] & [0.8, 1.0] \\
        \midrule
        AlexNet & 2.583 & 3.326 & 3.315 & 3.197 & 4.089 \\
        VGG-19 & 1.138 & 2.206 & 1.760 & 1.688 & 1.557 \\
        ResNet50 & 2.060 & 2.064 & 2.072 & 2.074 & 2.072 \\
        DenseNet121 & 0.686 & 0.693 & 0.692 & 0.692 & 0.693 \\
        \bottomrule
    \end{tabular}
    }
    \caption{Additional detailed results on density ratio v.s. HSF}
    \label{tab:dr_hsf2}
\end{table}

\subsubsection{Example Image from ImageNet for Density Ratio v.s. HSF.} We demonstrate two examples in Figure~\ref{fig:imagenetdata1_appendix} and Figure~\ref{fig:imagenetdata2_appendix} with their learned density ratios from DRL and their HSF values. The higher density ratios correspond with higher human selection frequencies.

\begin{figure*}[h]
        \centering
        \setlength{\tabcolsep}{-4pt}
        \begin{tabular}{ccc}
\includegraphics[height=4cm]{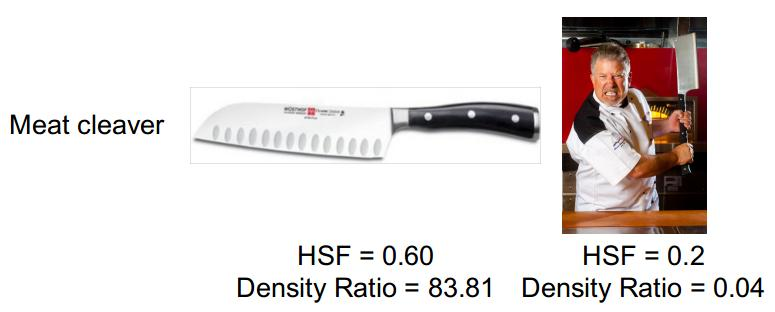}
      \end{tabular}
        \vspace{-0.1in}
             \caption{Example image from ImageNet with high and low human selection frequencies and corresponding high and low density ratios.}
     \label{fig:imagenetdata1_appendix}
    %  \end{tabular}
\end{figure*}

\begin{figure}[h]
        \centering
        \setlength{\tabcolsep}{-4pt}
        \begin{tabular}{ccc}
\includegraphics[height=4cm]{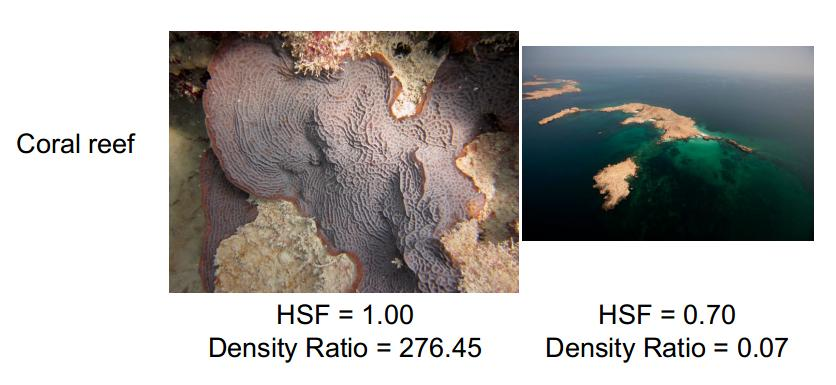}
      \end{tabular}
        \vspace{-0.1in}
             \caption{Example image from ImageNet with high and low human selection frequencies and corresponding high and low density ratios.}
     \label{fig:imagenetdata2_appendix}
    %  \end{tabular}
\end{figure}

\subsection{Additional DRST Results (for Section 3.2)}
\label{drst_results}
\begin{figure*}
        \centering
        \setlength{\tabcolsep}{-0pt}
        \begin{tabular}{ccccc}
Source: \\ &
\includegraphics[height=2.5cm, trim={0.5cm, 0.5cm, 0.0cm, 0.0cm},clip]{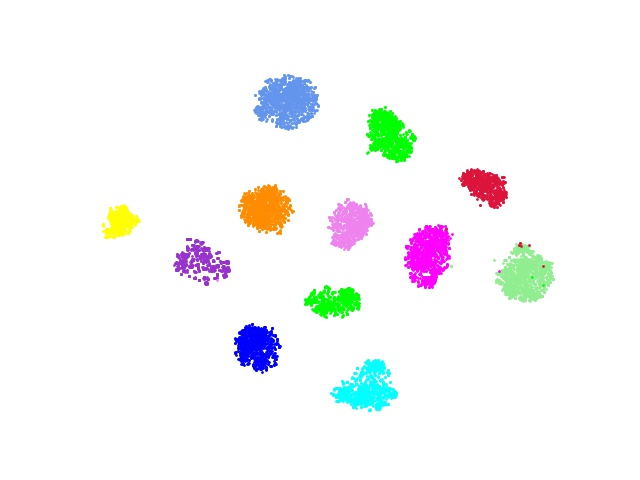}&
\includegraphics[height=2.5cm, trim={0.5cm, 0.5cm, 0.0cm, 0.0cm},clip]{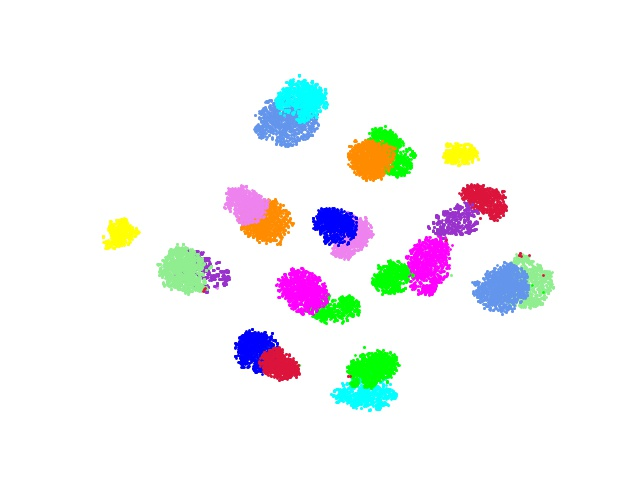}&
\includegraphics[height=2.5cm, trim={0.5cm, 0.5cm, 0.0cm, 0.0cm},clip]{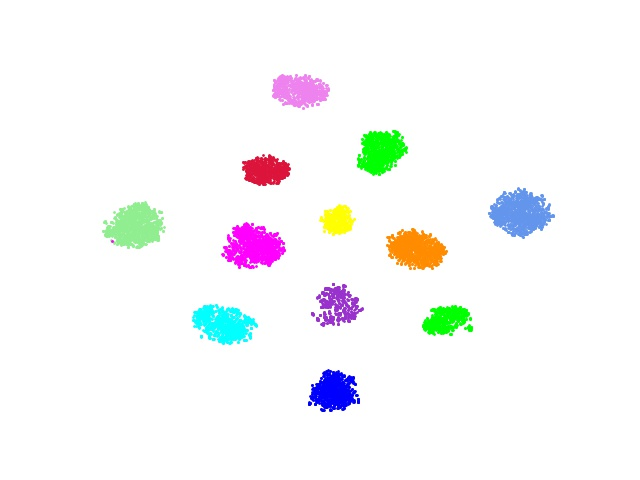}&
\includegraphics[height=2.5cm, trim={1cm, 0.5cm, 0.0cm, 0.0cm},clip]{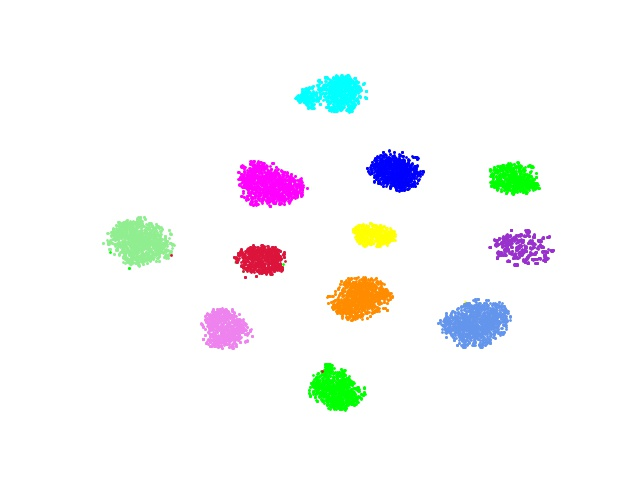}\\
Target: \\ &\includegraphics[height=2.5cm, trim={0.5cm, 0.5cm, 0.0cm, 0.0cm},clip]{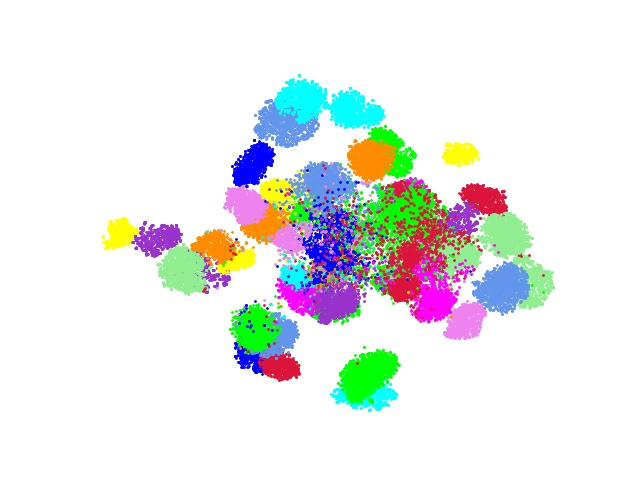}&
\includegraphics[height=2.5cm, trim={0.5cm, 0.5cm, 0.0cm, 0.0cm},clip]{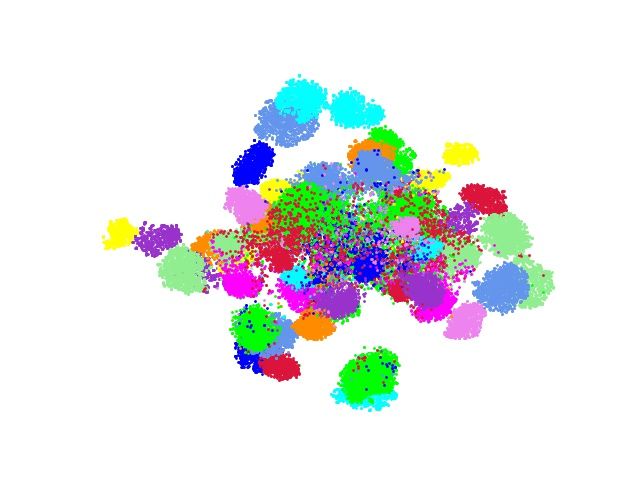}&
\includegraphics[height=2.5cm, trim={1cm, 0.5cm, 0.0cm, 0.0cm},clip]{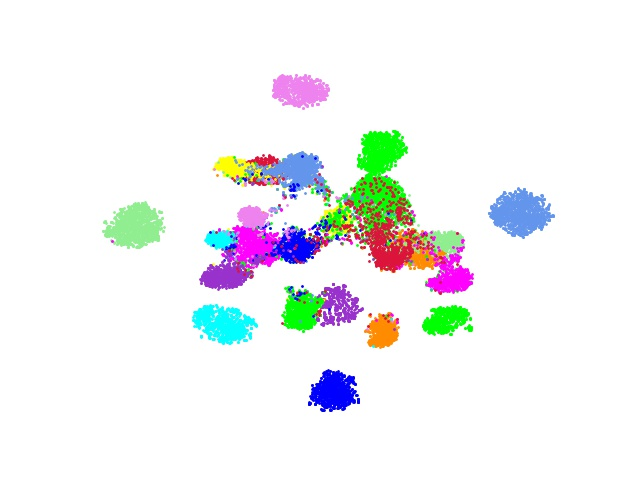}&
\includegraphics[height=2.5cm, trim={1cm, 0.5cm, 0.0cm, 0.0cm},clip]{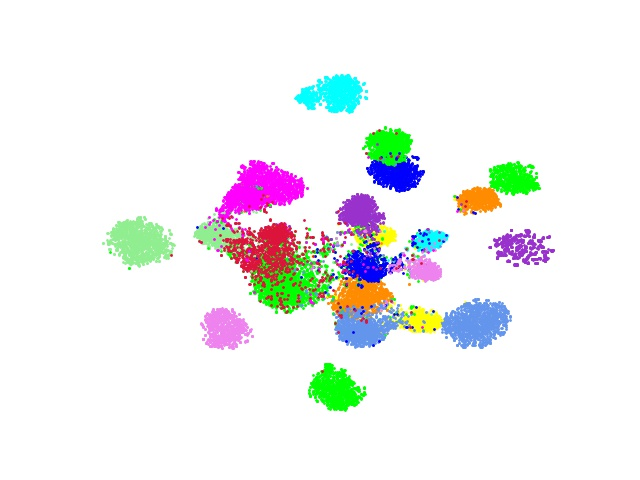}\\
&ASG &ASG+CBST &ASG+CRST &ASG+DRST
      \end{tabular}
        \vspace{-0.1in}
             \caption{TSNE visualization of the learned classifier using different methods. Using DRST, the classes are well-separated.}
    \label{fig:tsne}
\end{figure*}

\subsubsection{TSNE Comparison for DRST and Baselines on VisDA.} We demonstrate the TSNE plot of the learned decision boundaries for CBST, CRST and DRST in Figure~\ref{fig:tsne}. 

\subsubsection{Additional Attention Plots for DRST and Baselines on VisDA.} Figure  \ref{fig:attention_appendix}  and Figure \ref{fig:gradcam_correct} demonstrate additional model attention visualization by using Grad-Cam \footnote{Ramprasaath R Selvaraju, Michael Cogswell, Abhishek Das, Ramakrishna Vedantam, Devi Parikh, and Dhruv Batra. Grad-cam: Visual explanations from deep networks via gradient-based localization. In Proceedings of the IEEE international conference on computer vision, pages 618–626, 2017.}. 

\subsubsection{Example Target Data with Different Density Ratios on VisDA.} Figure~\ref{fig:diff_r_appendix} shows additional target examples with high and low density ratios. Our model is able to find noisy and less-represented image from the target data by estimating the density ratios. DRST would be more uncertain on those data.

\subsubsection{Additional DRSSL Results (for Section 3.3).}
We present more results on a different degree of data deficiency in Table \ref{tab:ssl_cifar_add} and Table \ref{tab:ssl_mnist_add}. We use even smaller number of source labeled data to start the SSL process.  We show the results for the two pairs of source and target domains in the paper: Source:CIFAR10/ Target: STL10 and Source:MNIST/ Target: SVHN. We show the result on both the source test set and the target test set.

\begin{table}[h]
\centering
\resizebox{0.48\textwidth}{11mm}{
\begin{tabular}{c|cc|cc}
\toprule
Labeled Samples & \multicolumn{2}{c|}{250} & \multicolumn{2}{c}{40} \\ 
\midrule
Test Set & CIFAR10 &  STL10 & CIFAR10 & STL10 \\ \midrule
Fixmatch & 65.70 & 47.92  & 50.98 & 23.50 \\ 
DRSSL    & 93.58 & 66.01  &  92.50 & 63.69 \\ \bottomrule
\end{tabular}
}
\caption{Additional results on CIFAR10$\rightarrow$STL10}
\label{tab:ssl_cifar_add}
\end{table}

\begin{table}[b]
\centering
\resizebox{0.48\textwidth}{11mm}{
\begin{tabular}{c|cc|cc}
\toprule
Labeled Samples & \multicolumn{2}{c|}{400} & \multicolumn{2}{c}{40} \\ 
\midrule
Test Set &  MNIST & SVHN & MNIST & SVHN \\ \midrule
Fixmatch & 99.25 & 25.62 & 97.26 & 25.84 \\ 
DRSSL    & 99.29 & 32.19 & 97.28 & 27.06 \\ \bottomrule
\end{tabular}
}
\caption{Additional results on MNIST$\rightarrow$SVHN}
\label{tab:ssl_mnist_add}
\end{table}

\begin{figure*}[h]
        \centering
        \setlength{\tabcolsep}{-4pt}
        \begin{tabular}{ccc}
    \includegraphics[height=2.5cm, trim={1cm, 2cm, 0.5cm, 1cm}, clip]{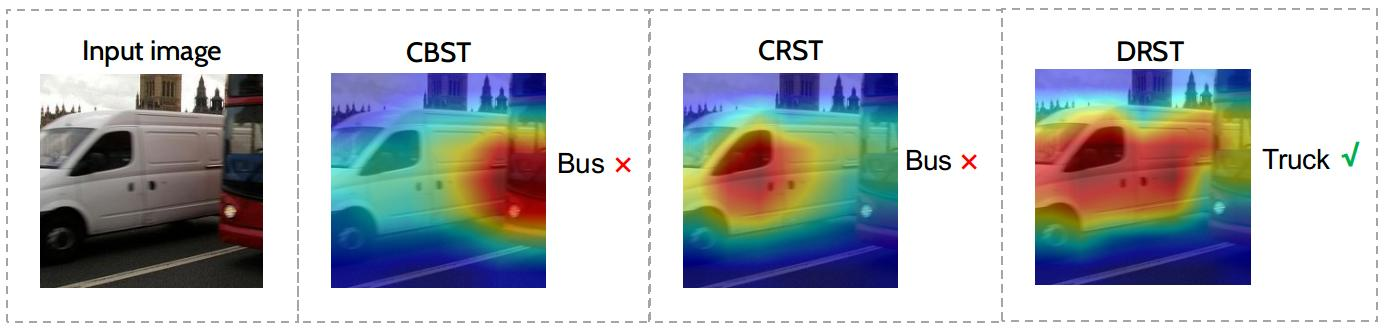} \\
    \includegraphics[height=10cm]{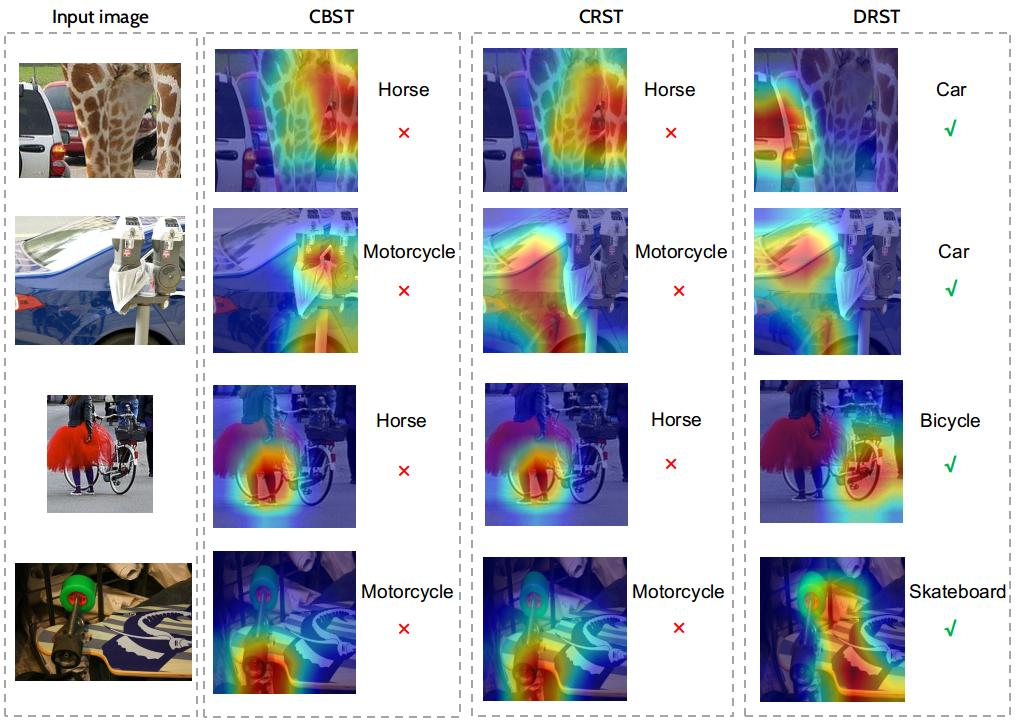}
      \end{tabular}
        \vspace{-0.1in}
             \caption{Model attention visualized using Grad-Cam. We also show the predicted labels by different methods. The first row shows that DRST captures the  shape features of the image better. DRST can also capture the domain knowledge well. For example, the second row input image contains a giraffe and a car. However, giraffe is not a existing label for VisDA2017. While CBST and CRST capture the wrong information, DRST is able to correctly capture the domain information.}
     \label{fig:attention_appendix}
    %  \end{tabular}
\end{figure*}
%\cite{selvaraju2017grad}

\begin{figure*}[h]
\vspace{-10pt}
    \centering
    \includegraphics[width=0.9\textwidth]{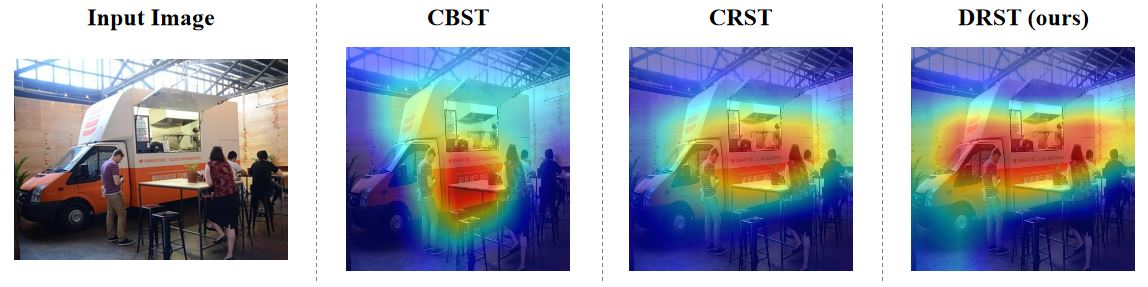}
    \caption{Model attention on a correctly predicted example by baseline methods and our method. Ours has better reception field.}
    \label{fig:gradcam_correct}
\end{figure*}

\begin{figure*}[h]
        \centering
        \setlength{\tabcolsep}{-4pt}
        \begin{tabular}{ccc}
\includegraphics[height=10cm]{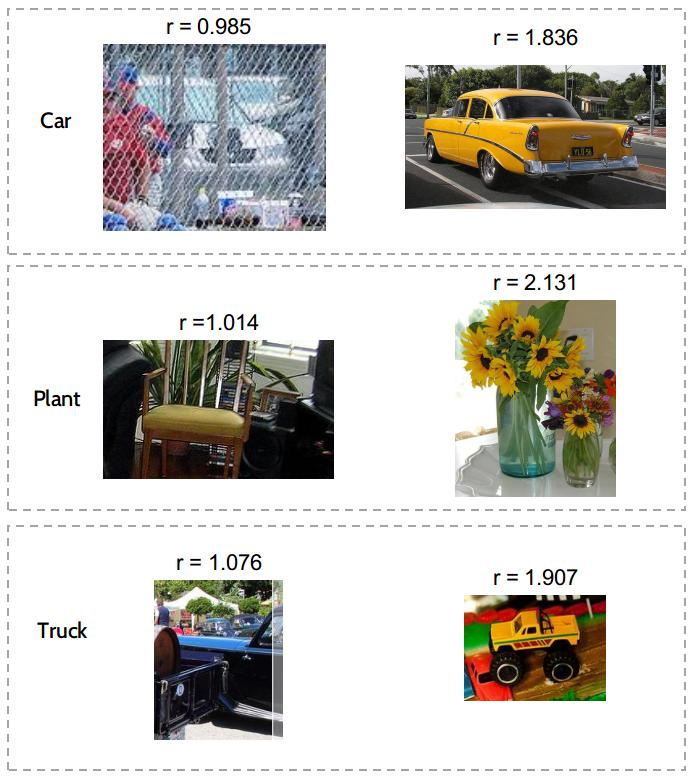}
      \end{tabular}
        \vspace{-0.1in}
             \caption{Additional examples for density ratio estimation for different categories. We can observe that data less well-represented in the source data has much lower density ratio. This shows that our learned density ratio is a good measure of the level of representation of data in source and target domains.}
     \label{fig:diff_r_appendix}
    %  \end{tabular}
\end{figure*}

\section{Experiment details}
\label{appendix_details}
Here we include the experimental details that was not shown in Section \ref{sec:exp} due to space limit. 

\subsection{Metric explanation}
We calculate Brier score as the mean squared difference between the predicted probability $p$
assigned to the possible outcome and the actual outcome $y$: $BS = \frac{1}{n}\sum\limits _{i=1}^{n}\sum\limits _{j=1}^{m}(p_{ij}-y_{ij})^2 \,\!$. ECE is calculated as $\sum_{j=1}^{J}\frac{B_j}{N}|\text{acc}(B_j) - \text{conf}(B_j)|$, where $B_j$ is a set of predictions binned by confidence values, $\text{acc}(B_j)$ is the average accuracy of the $B_j$ , and $\text{conf}(B_j)$ is the average confidence of the most likely label. 

\subsection{Computation resources}
All of our training experiments are done on the DGX V100 Tesla V100 GPUs with 32GB memory. The main packages and corresponding versions we use are: Python 3.6, PyTorch 0.4.0, CUDA 10.1. 

\subsection{Details for section 3.1}
We train DRL on Office31 and OfficeHome using the ResNet50 backbone, and use the ResNet101 backbone for VisDA. DRL on ImageNetV2 uses the DenseNet121 backbone. For each task, we use the same backbone for the source model and the TS model to make comparison fair. TS models adopt a temperature value of 1.5, and is scaled by using the target dataset containing both images and labels. The DRL models we train use different update frequencies for the density ratio estimator and the classifier. The classifier is trained for every batch iteration, and the density ratio estimator is trained once per 5 batch iterations and we guarantee that the estimator sees all of the target domain data at least once. For training on Office31, OfficeHome and ImageNet, we use the SGD optimizer with learning rate selected from $[0.03, 0.01,0.001, 0.0001]$, momentum $0.9$ and weight decay rate of $0.0001$.

We have done experiments on ImageNet using four different network architectures: AlexNet, VGG-19, ResNet50 and DenseNet121. The training details follow the official PyTorch training process. The models are not trained from scratch but rather use pretrained models as the starting point. For AlexNet, VGG-19 and ResNet50, we use a learning rate of $10^{-4}$; For DenseNet121, the learning rate is $10^{-6}$. Note that when comparing the scores where there consist of the TS (temperature scaling) baseline (such as Figure 4 in main text), we only use half of the ImageNetV2 dataset to do the evaluation. The other half of the dataset is used to train the TS model. This is for the fair comparison of TS and the other models so that they all cannot access the test data during the training process. 

The datasets and models we use are publicly open and does not contain personally identifiable information or offensive contents.

\subsection{Details for section 3.2}
In this subsection, we focus on self-training for UDA. We follow the same implementation as CBST and only change the model and few hyperparameter values. We set batch size as 16, use the SGD optimizer with learning rate $10^{-5}$ and momentum 0.9. The initial value of source data portion is $6.5\%$ and we add $0.85\%$ of source data number of data into the training set every epoch. The maximum portion is set as $16.5\%$.

\subsection{Details for section 3.3}
\label{cdssl}
Another semi-supervised learning setting with domain gaps also exists, which is semi-supervised domain adaptation (SSDA). The reasons why we test on cross-domain semi-supervised learning (CDSSL) setting instead of SSDA are: 1) the two common definitions (see details in \footnote{K. Saito, D. Kim, S. Sclaroff, T. Darrell and K. Saenko, "Semi-Supervised Domain Adaptation via Minimax Entropy," 2019 IEEE/CVF International Conference on Computer Vision (ICCV), 2019.} and \footnote{David Berthelot, Rebecca Roelofs, Kihyuk Sohn, Nicholas Carlini, and Alex Kurakin. Adamatch: A unified approach to semi-supervised learning and domain adaptation. CoRR, abs/2106.04732, 2021.}, respectively) in SSDA are both not readily to be plugged in by our technique, which means it is difficult to directly compare with SSDA methods. 2) CDSSL is more challenging and realistic. Specifically, CDSSL aims to use few labeled source training examples and many unlabeled target training examples to predict on source testing examples and target testing examples. Different from SSDA, in CDSSL source data is partially labeled and the target data is unlabeled.

The reason of no more baselines is that our implementation is a plugin for FixMatch, thus we use FixMatch as a baseline. For CDSSL, we do not identify other recent peer methods. Under the single domain setting, FixMatch trains the model using source labeled data and source unlabeled data. However, under the cross-domain setting, we train the model using source labeled data and target unlabeled data. We follow the implementation of Fixmatch and use the same augmentation methods. The unlabeled dataset uses all of the target domain train data, while the labeled dataset samples the same number of data for every class from the source domain data. 

We test both the source test data performance and the target test data performance, to evaluate label efficiency under different settings. We tested the performance when using different pretrained models for DRSSL. The pretrained models are achieved by using Fixmatch but under different settings, including the source-only setting (original Fixmatch setting) and the cross-domain setting (the setting which we use). We find that for CIFAR10$\rightarrow$STL10 task, the source-only setting helps to achieve better final performance ($5\%$ more) while for MNIST$\rightarrow$SVHN, the two settings yield similar performance. 

For the CIFAR10$\rightarrow$STL10 task, note that the ten classes in two datasets are different. CIFAR10 and STL10 only have 9 classes in common, thus we eliminate the `frog' samples in CIFAR10 and the `monkey' samples in STL10. Also note that we regard the `automobile' class in CIFAR10 and `car' class in STL10 as the same. We also match the order in which the classes are represented.

\section{Potential Negative Societal Impacts} 
This paper do not explicitly study any fairness issues within our method. But when the data is human-related, our algorithm may suffer from unfair predictions as conventional deep learning algorithms. Our future work include incorporating fairness constraints into the DRL framework. In this paper, our method mostly focuses on computer vision applications and should not be applied to safety-critical applications using the current form. Therefore, our future work also include investigating how to achieve safety guarantees %of the performance 
when data is of high-dimension.

\section{Code Repository}
Code is available in this repository: https://anonymous.4open.science/r/Deep-Distributionally-Robust-Learning-for-Calibrated-Uncertainties-under-Domain-Shift-7C2E.
